# Supplementary material for: Measurement of the forward $Z$ boson production cross-section in $pp$ collisions at $\sqrt{s}$ = 7 TeV
Source: arXiv:1505.07024 source file (2015-08-20)
Supplement: Supplementary file 1 [file supplementary-app.tex]

\clearpage

\section{Supplementary material for LHCb-PAPER-2015-001}
\label{sec:Supplementary-App}

This appendix contains supplementary material that will posted
on the public cds record but will not appear in the paper.

\begin{figure}[tbh]
  \begin{center}
    \includegraphics[width=\linewidth]{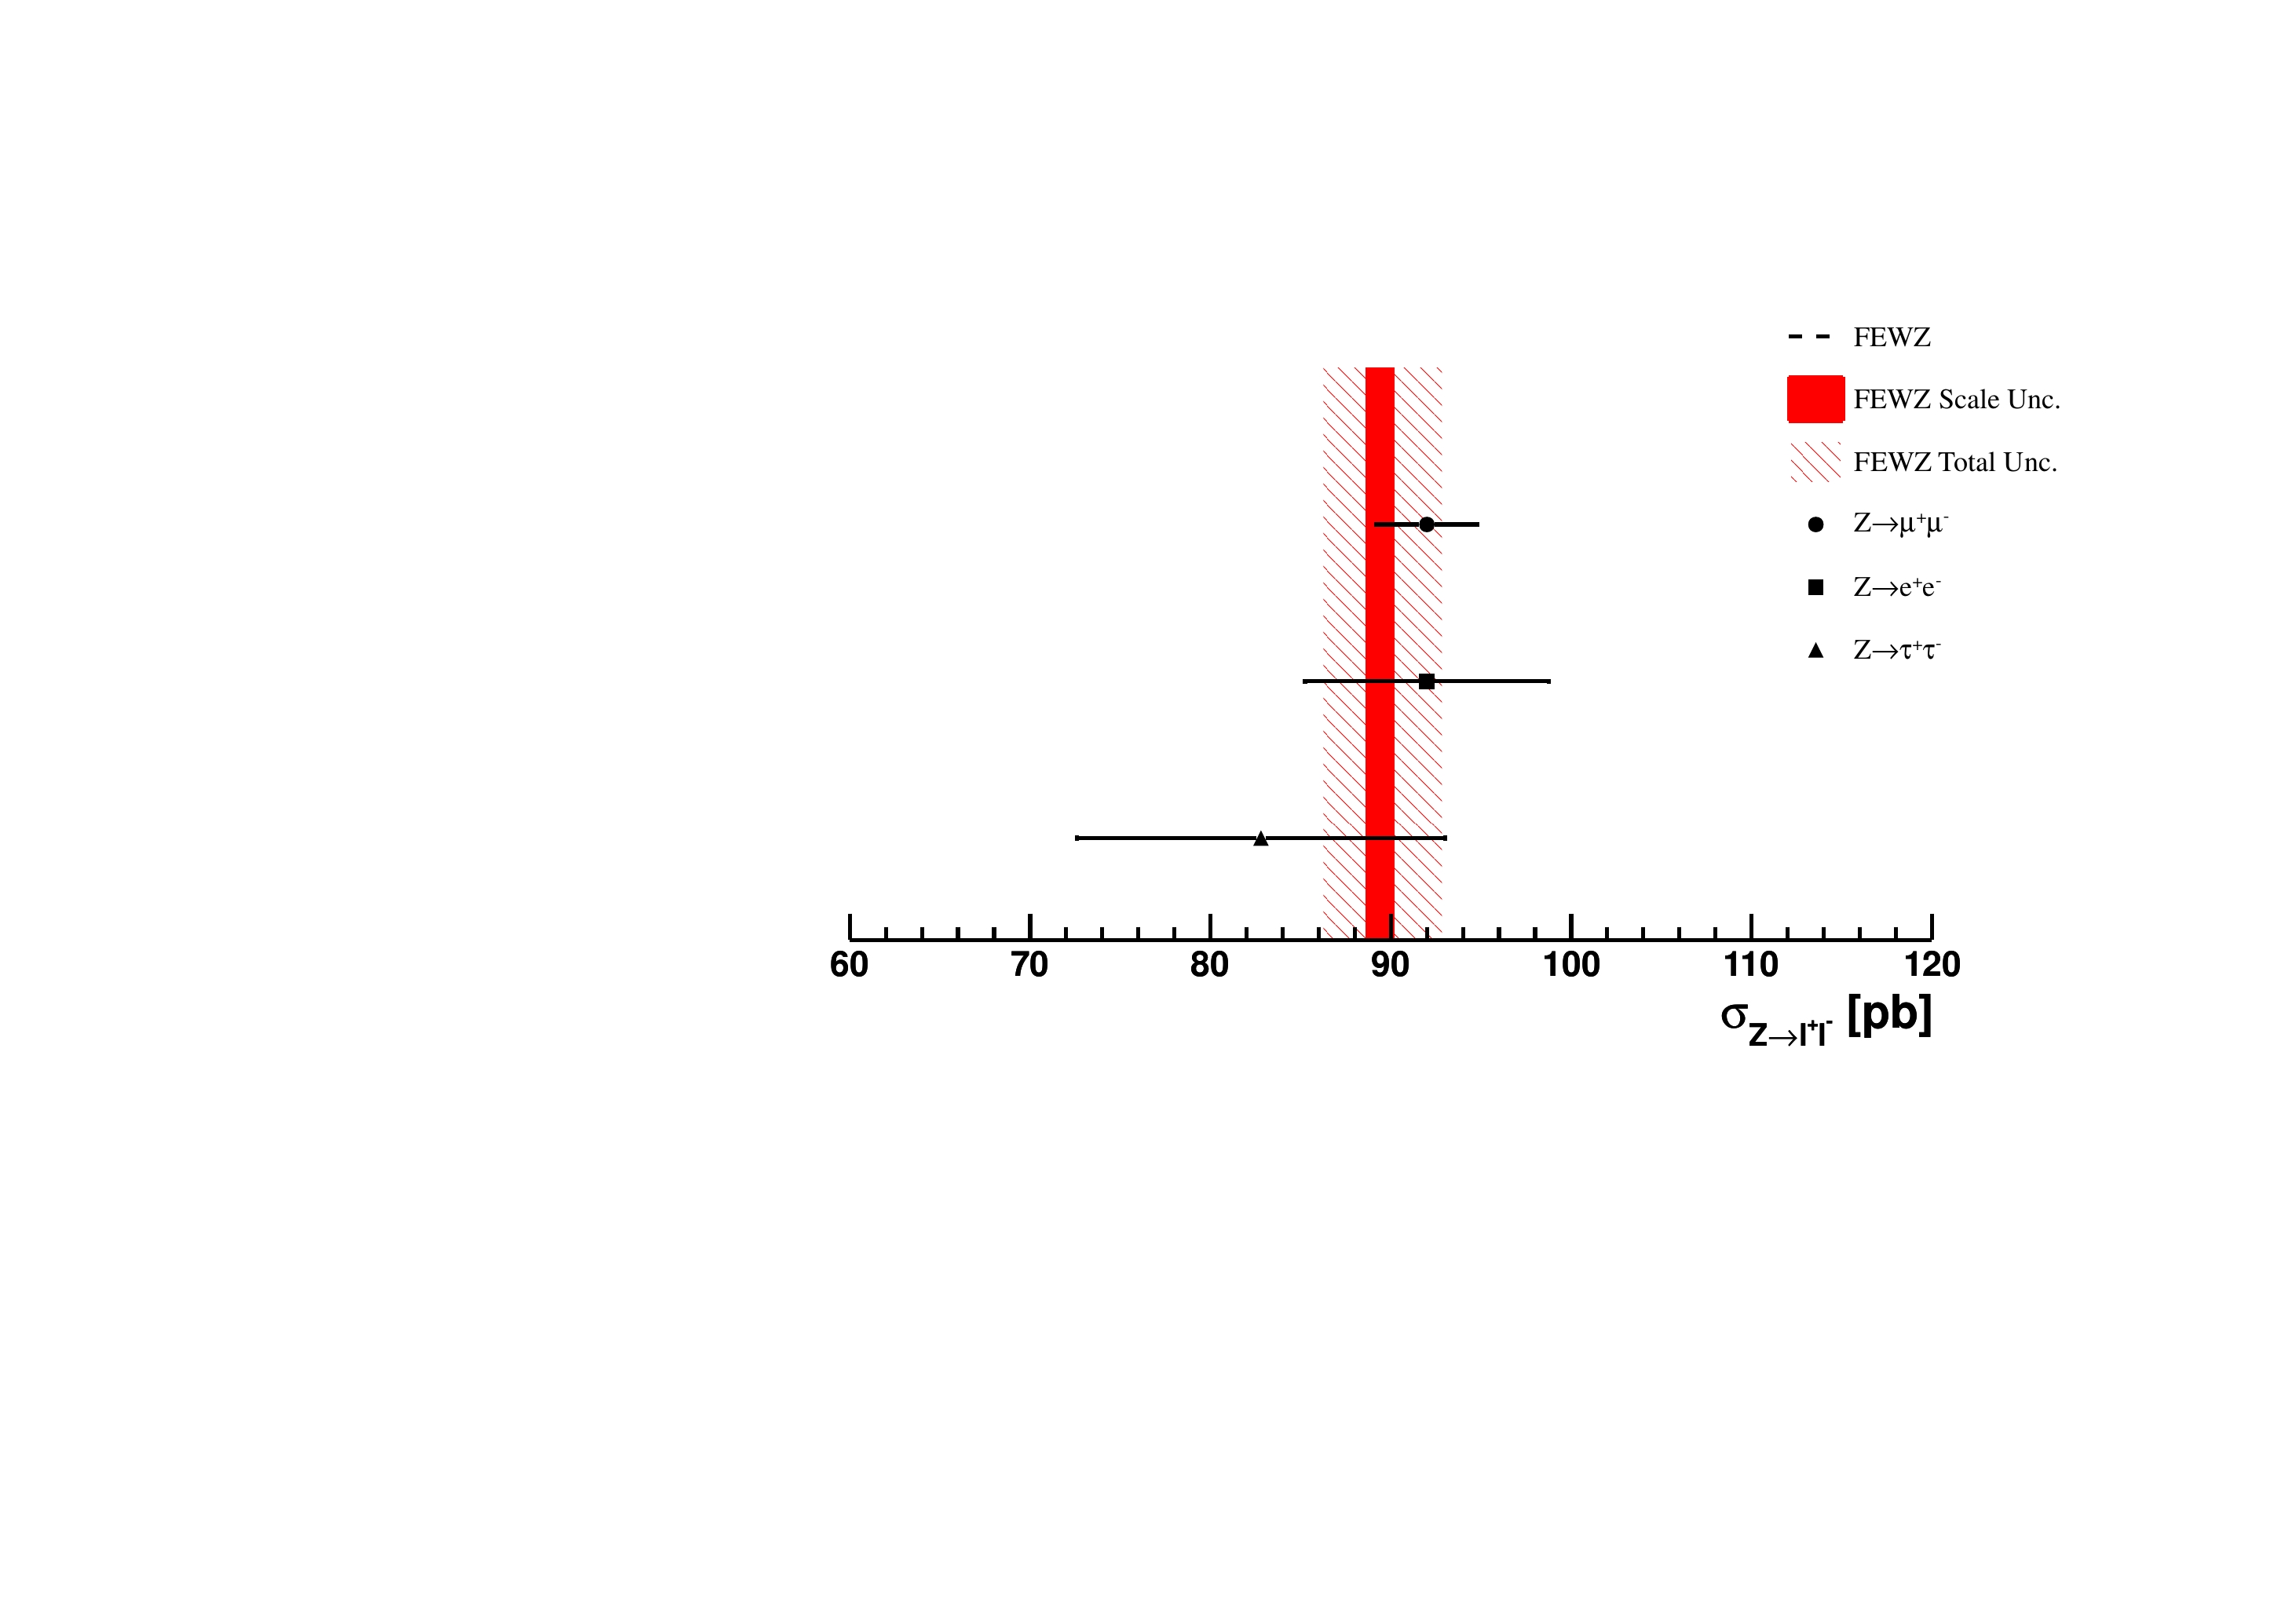}
  \end{center}
  \caption{Comparison of \lhcb \PZ cross-section measurements to theoretical prediction. The uncertainty due to the beam 
           energy is not displayed.}
  \label{fig:univ}
\end{figure}

\clearpage

\begin{figure}[tbh]
  \begin{center}
    \includegraphics[width=\linewidth]{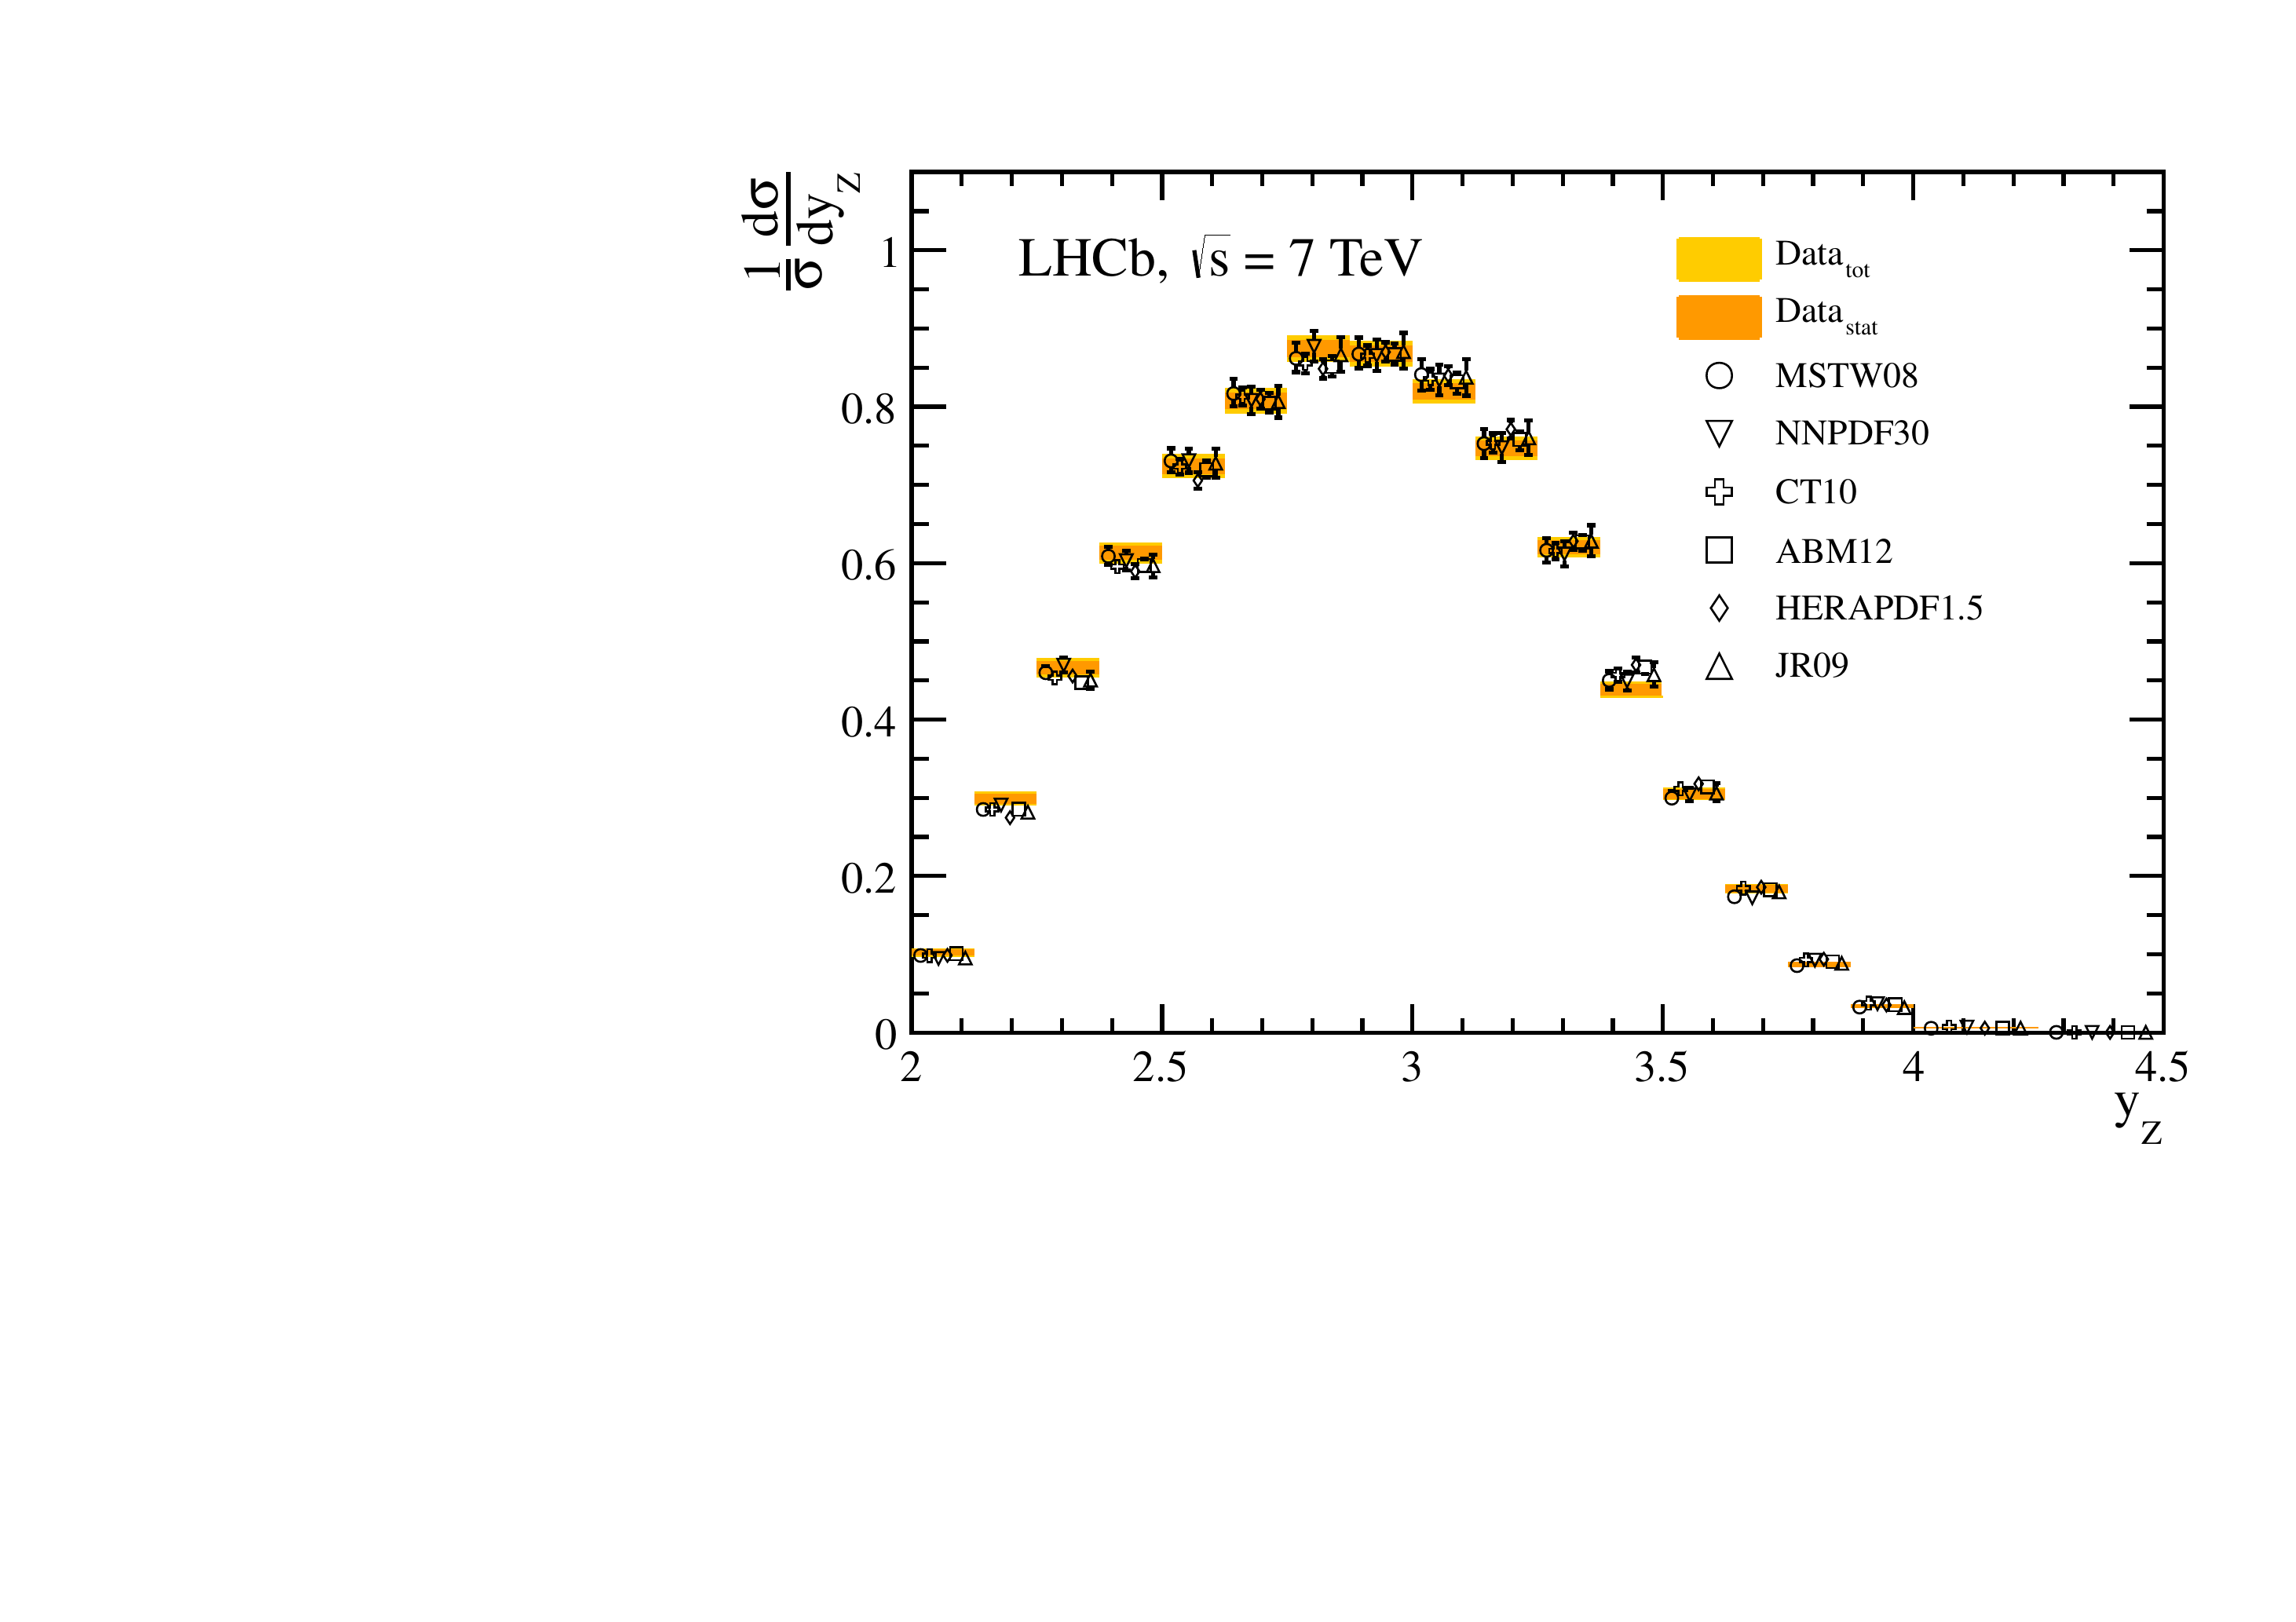}
  \end{center}
  \caption{
    %\small %captions should be a little bit smaller than main text
   Normalised differential cross-section as a function of $y_{Z}$. The 
shaded (yellow) bands indicate
   the measurements. These are compared to \fewz with various PDF sets.
  }
  \label{fig:diffxsecYfewznorm}
\end{figure}

\clearpage

\begin{figure}[tbh]
  \begin{center}
    \includegraphics[width=\linewidth]{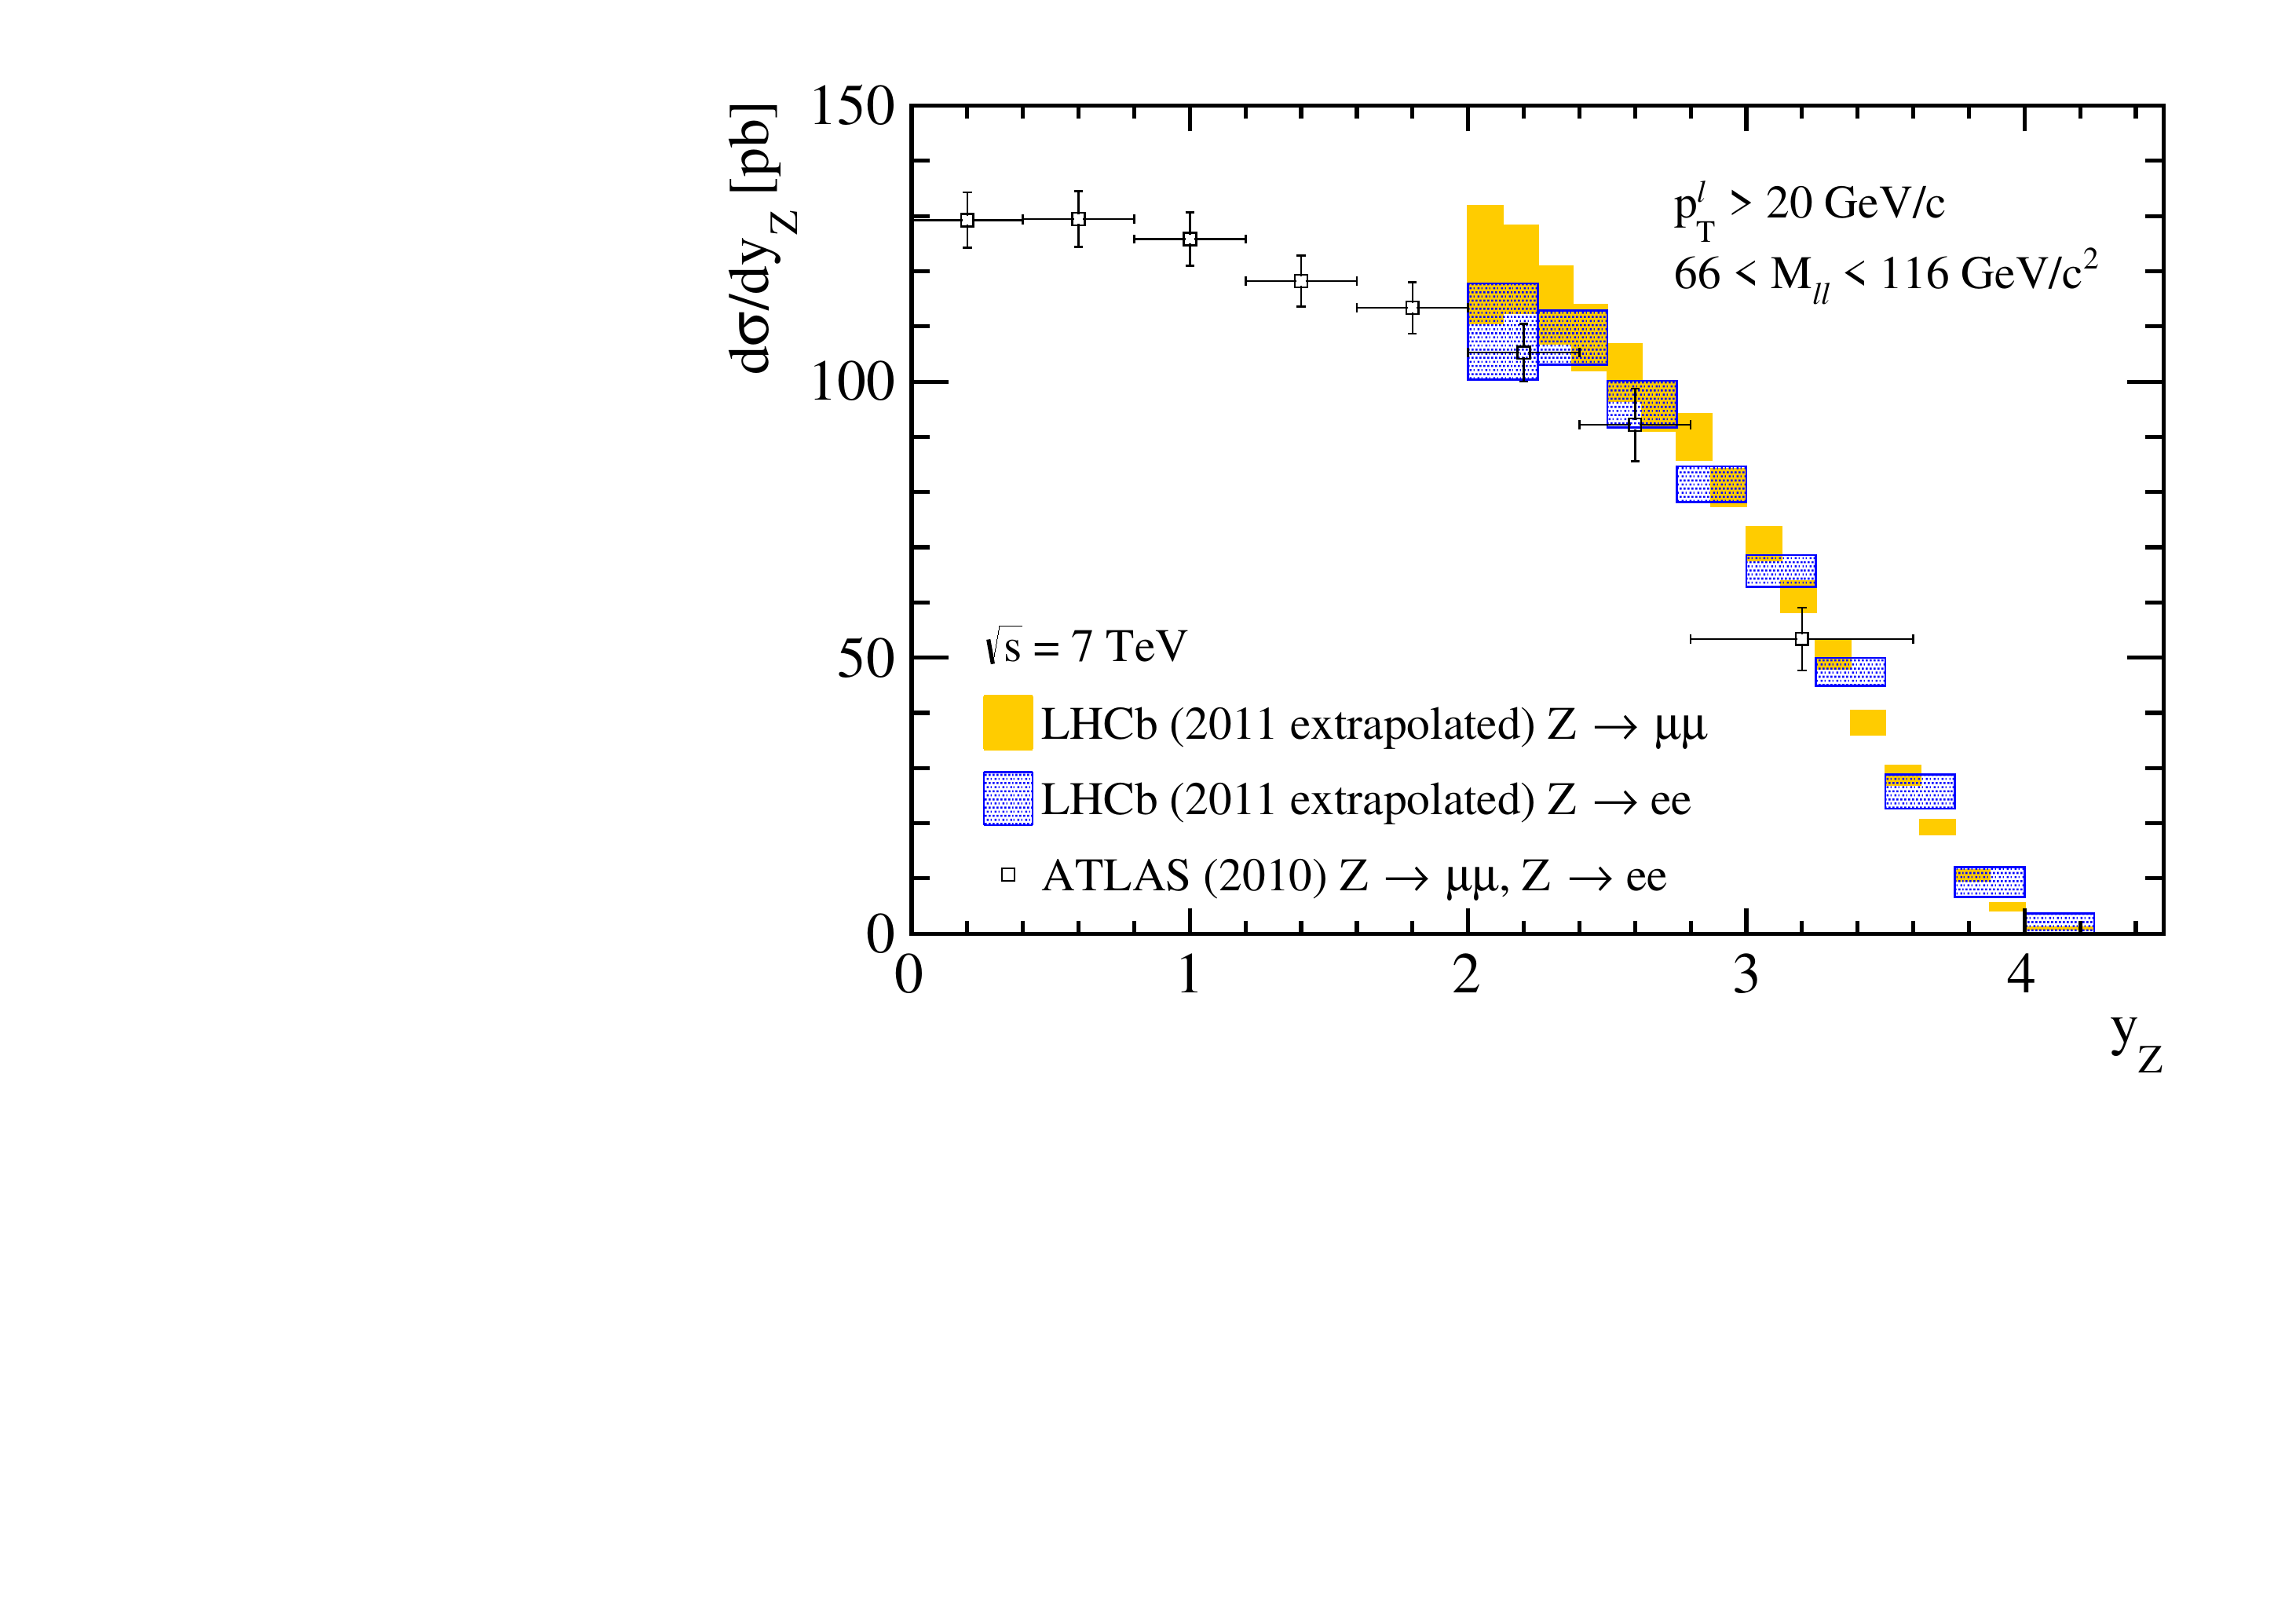}
  \end{center}
  \caption{Extrapolation of \lhcb \PZ boson cross-section measurements to the ATLAS fiducial volume (muons with $\pt > 20$ \gevc and invariant mass $66<M_{\mu\mu}<116$ \gevcc)~\cite{atlaswz}.}
  \label{fig:extrap}
\end{figure}

\clearpage

\begin{figure}[tbh]
  \begin{center}
    \includegraphics[width=\linewidth]{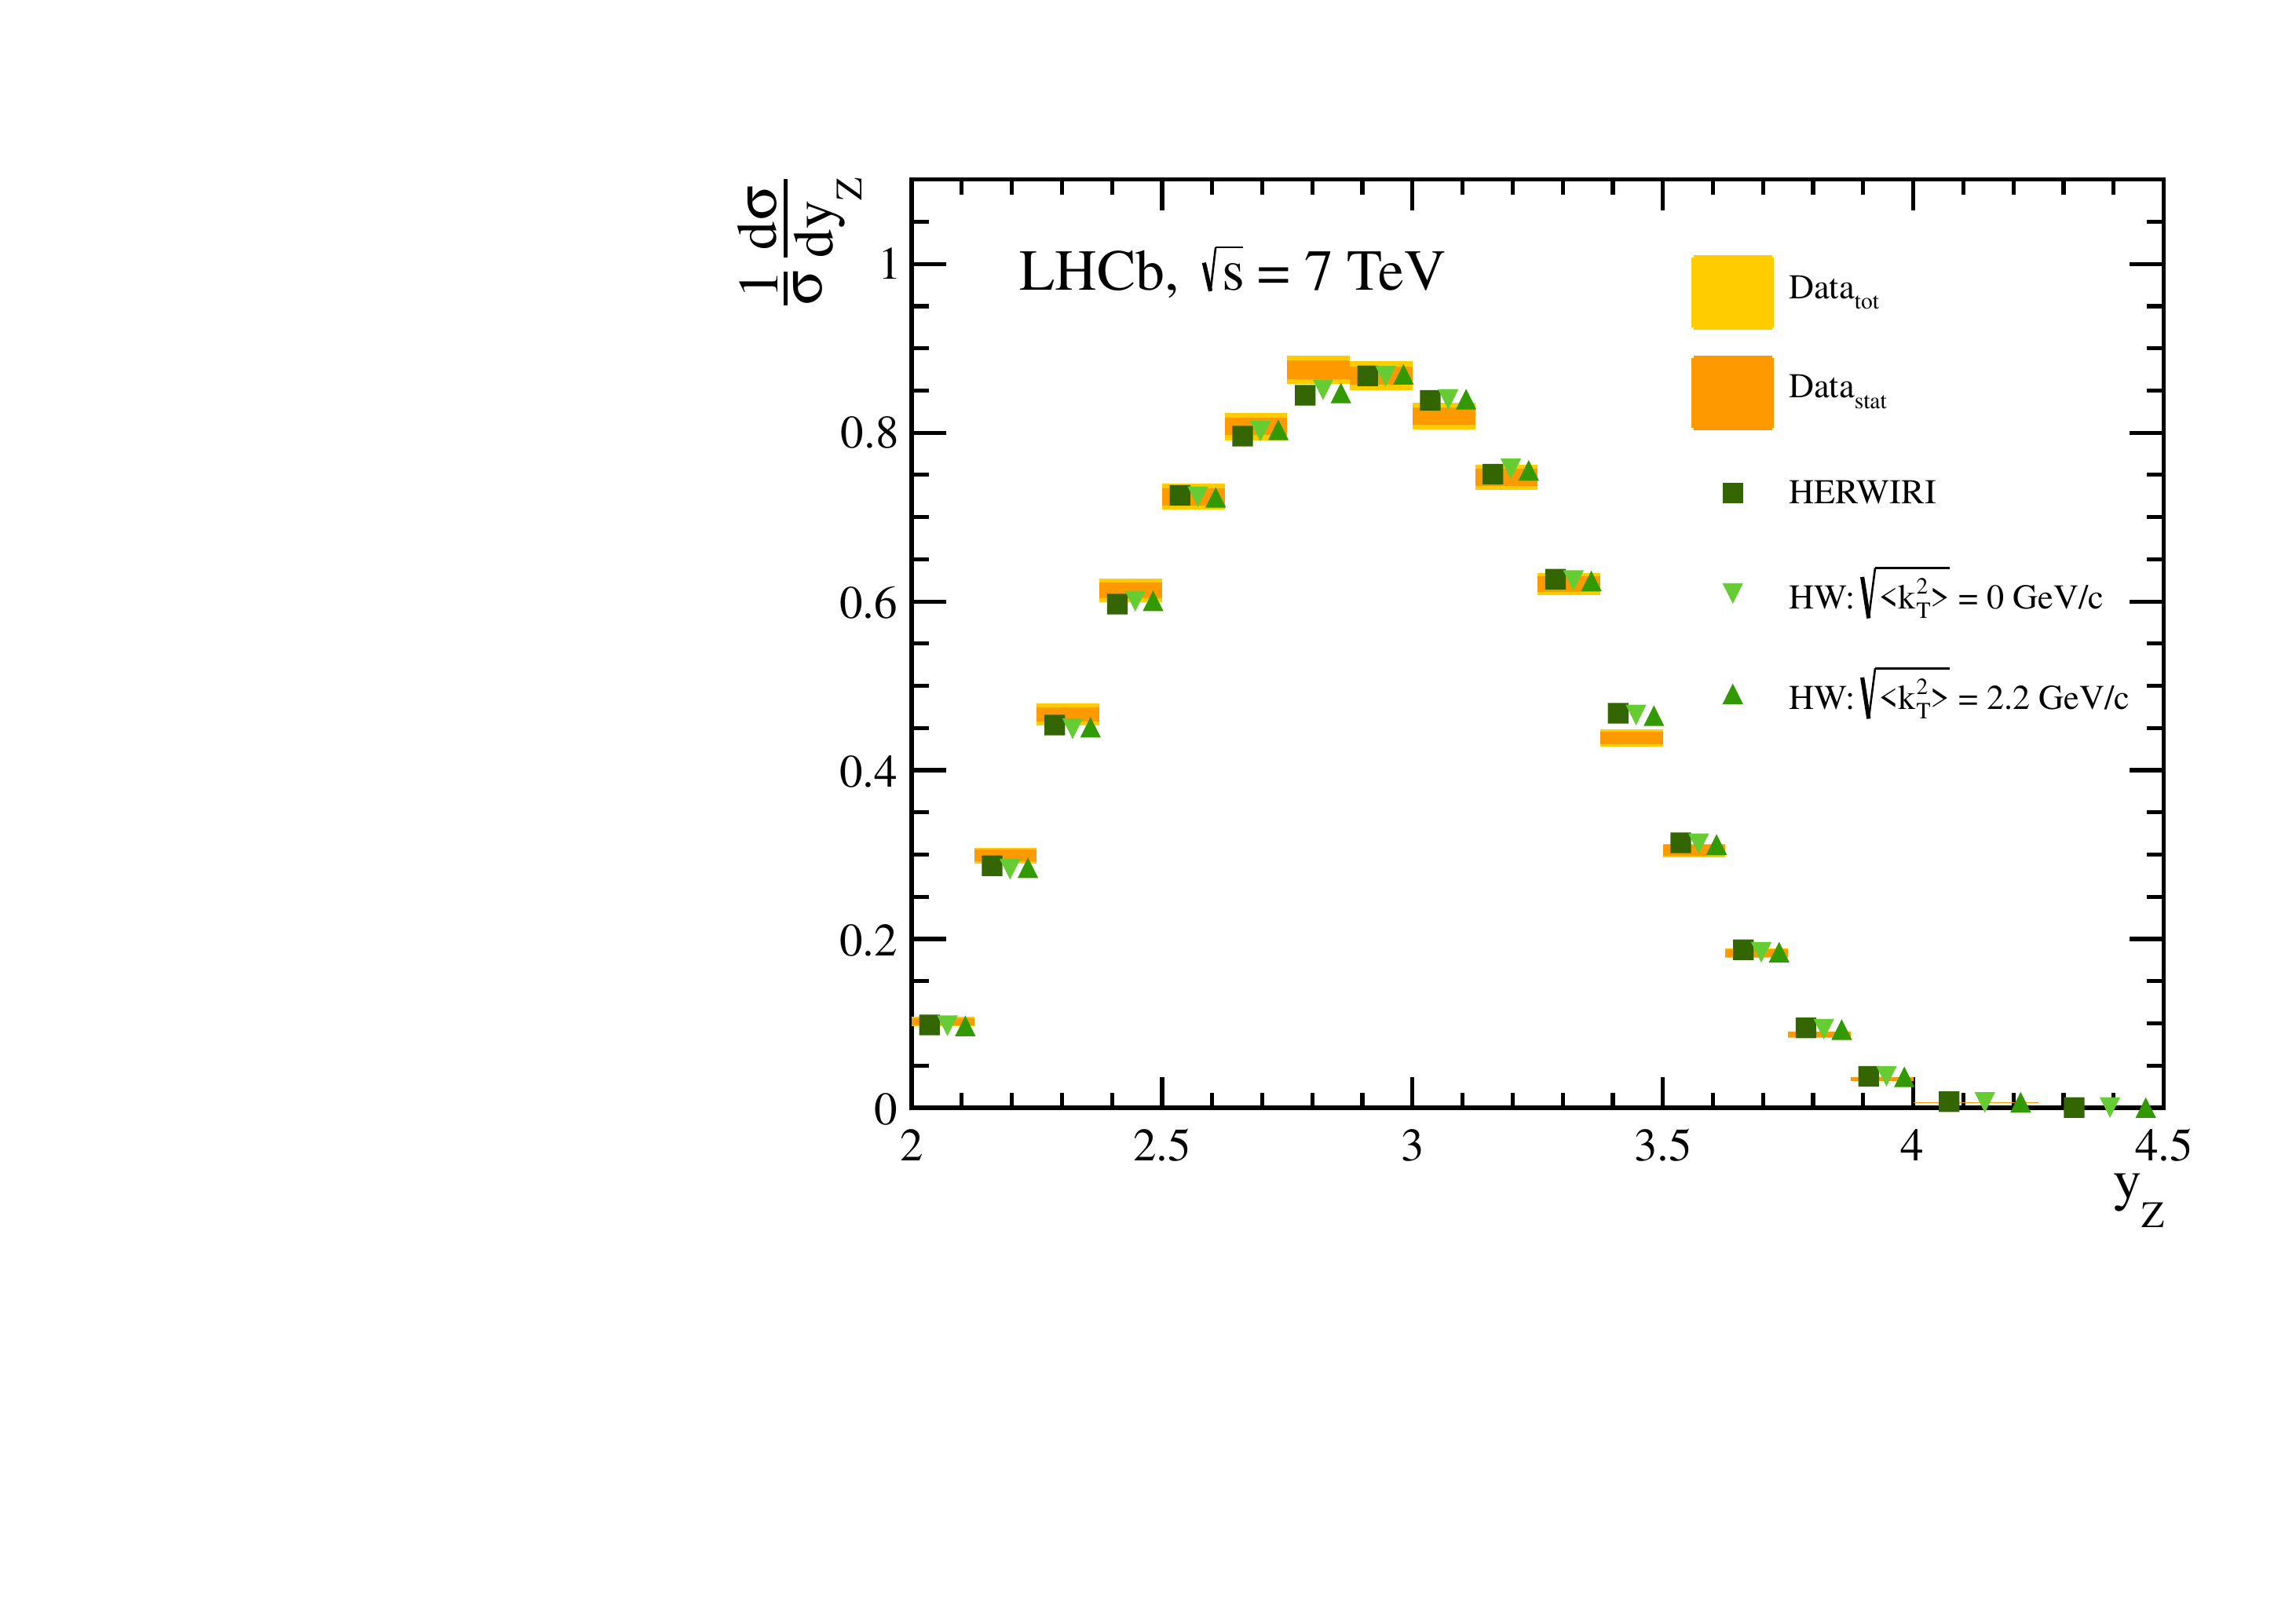}
  \end{center}
  \caption{
    %\small %captions should be a little bit smaller than main text
   Normalised differential cross-section as a function of \PZ boson $y$. 
The shaded (yellow) bands indicate
   the measurements, which are compared to \mc@nlo + \herwiri (HERWIRI) and 
\mc@nlo + \herwig (HW).
\herwig is configured with two choices of the root mean-square-deviation of 
the intrinsic $k_{T}$ distribution, 0 and 2.2 \gevc.
  }
  \label{fig:diffxsecYHERWIRI}
\end{figure}

\clearpage

\begin{figure}[tbh]
  \begin{center}
    \includegraphics[width=\linewidth]{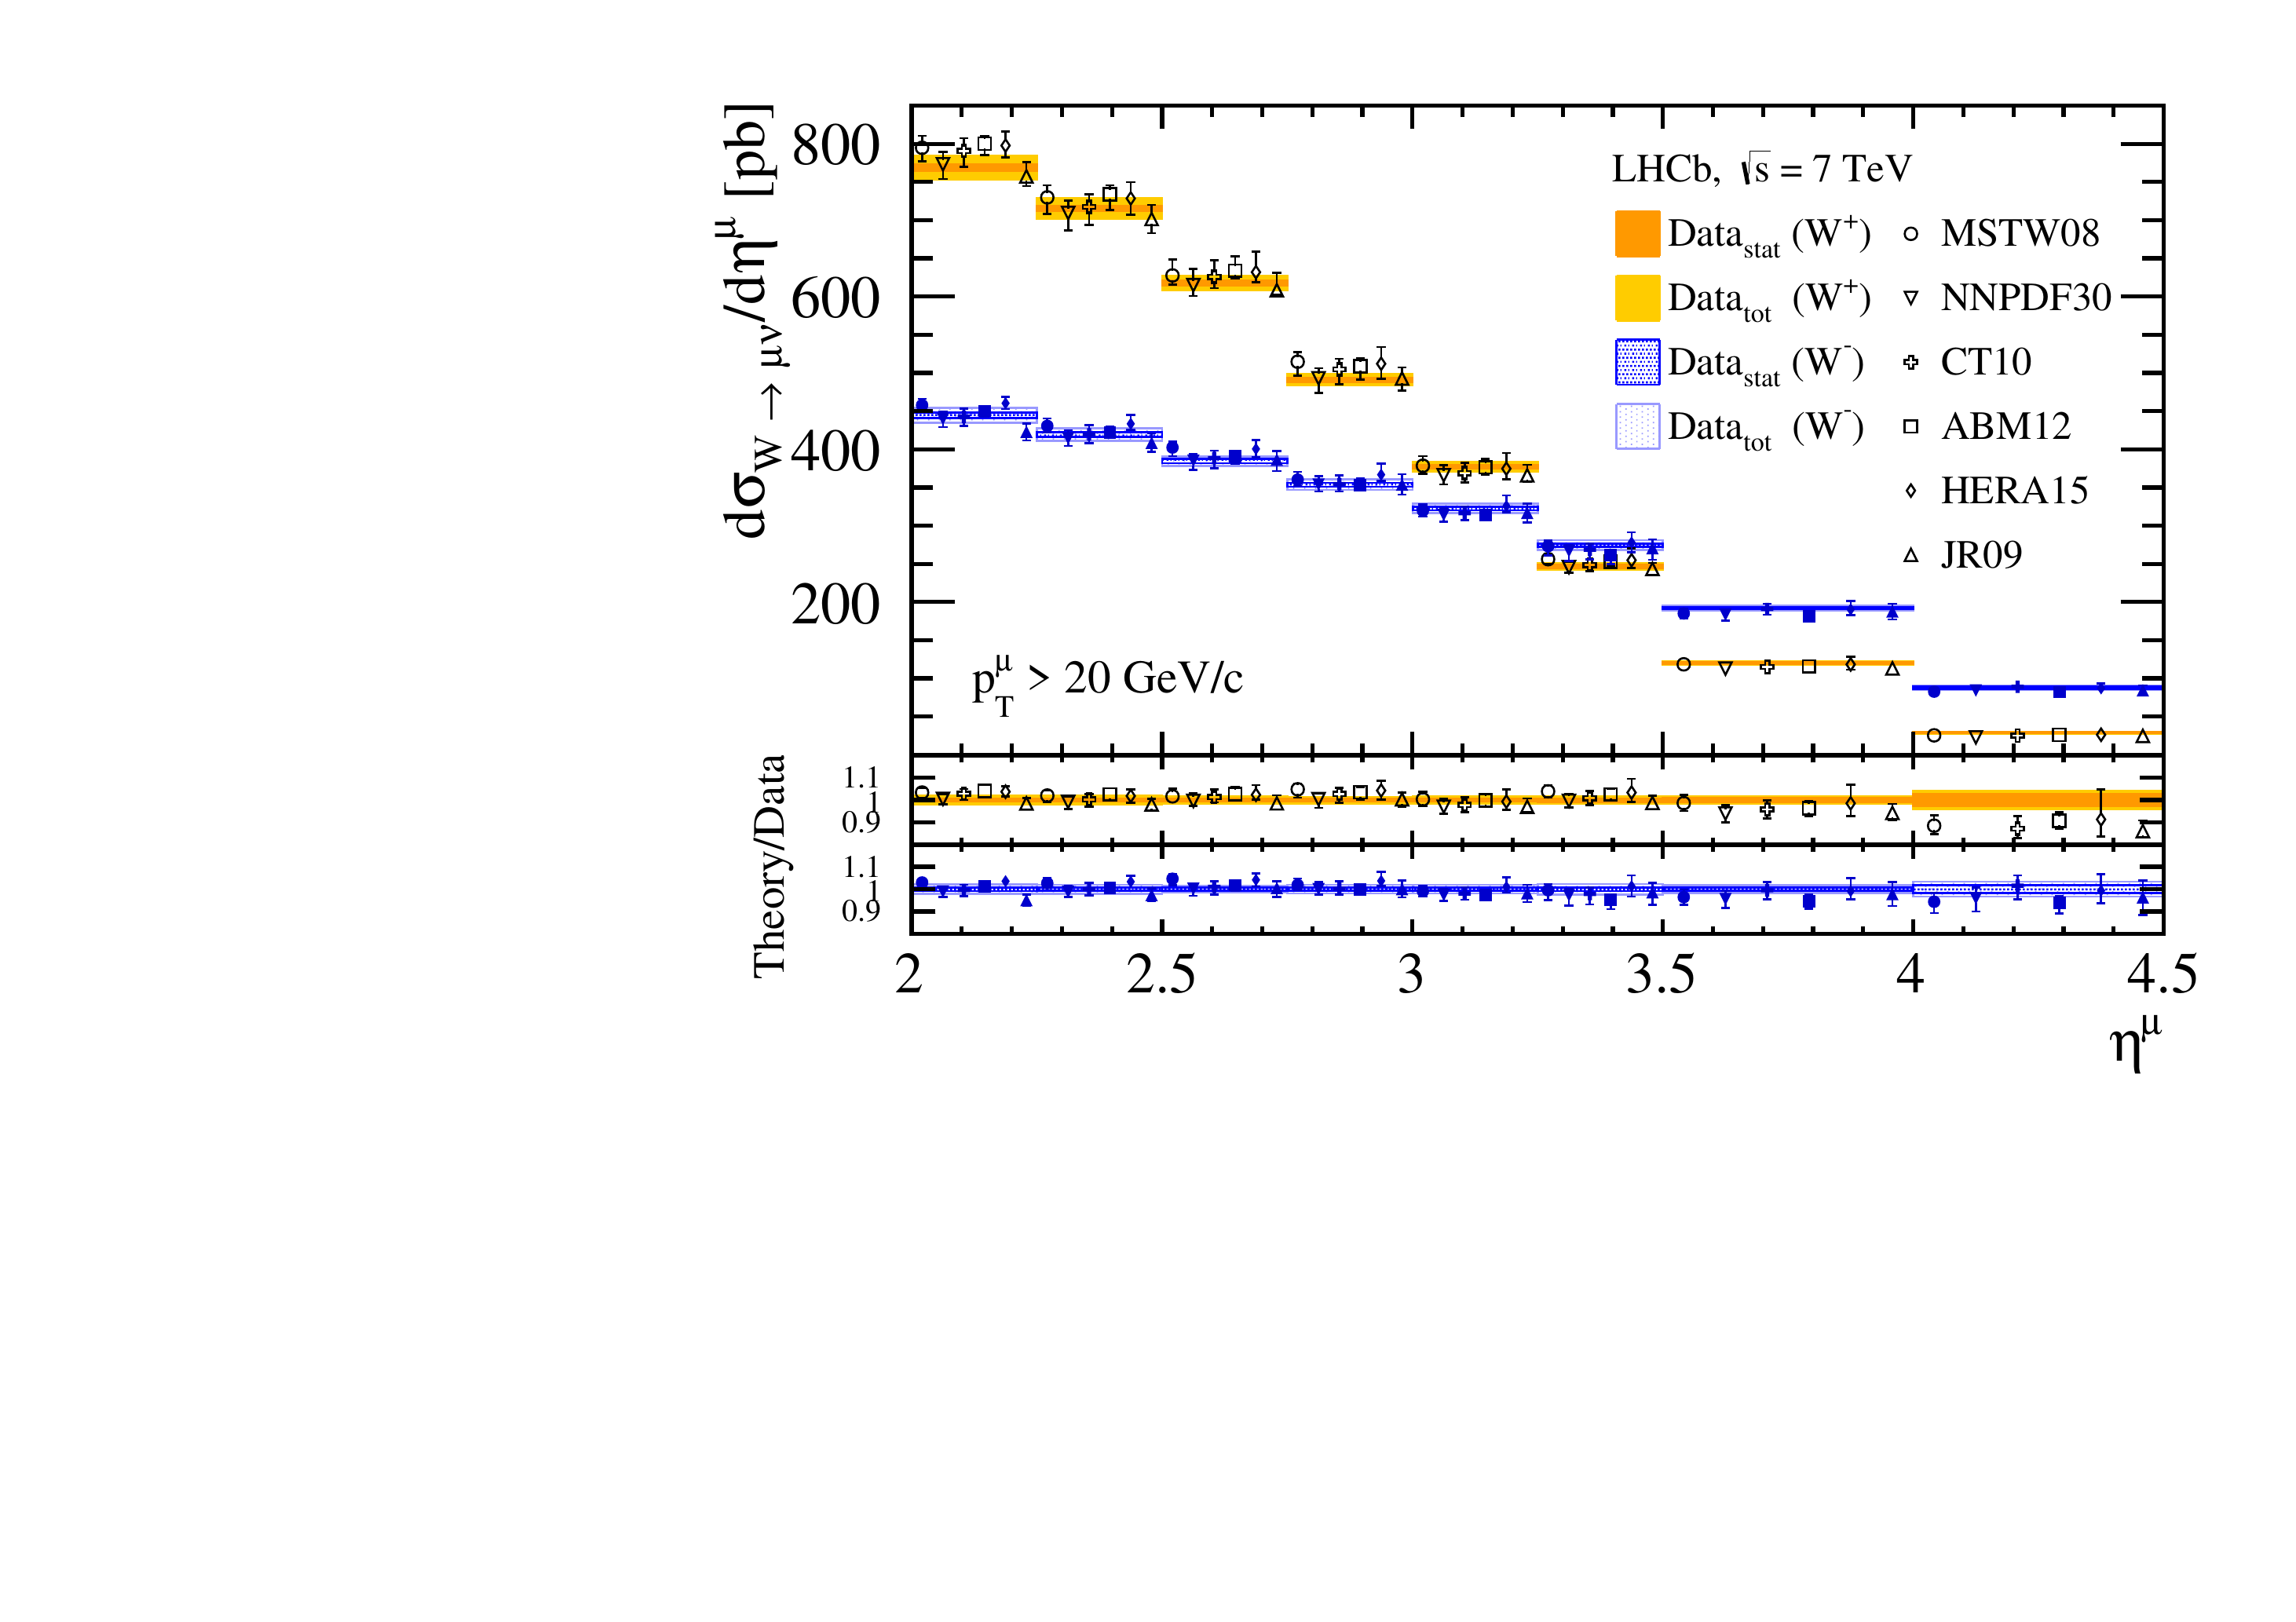}
  \end{center}
  \caption{
          Differential $W^{+}$ and $W^{-}$ cross-sections as a function of 
muon $\eta$. Measurements, represented
          as bands corresponding to the statistical (orange (blue) for $W^{+}$ ($W^{-}$)) and total
          (yellow (light blue) for $W^{+}$ ($W^{-}$)) uncertainty, are compared to NNLO predictions with
          different parameterisations of the PDFs (black (blue) markers for $W^{+}$ ($W^{-}$)), displaced
          horizontally for presentation.
  }
  \label{fig:csw}
\end{figure}  

\clearpage

\begin{figure}[tbh]
  \begin{center}
    \includegraphics[width=\linewidth]{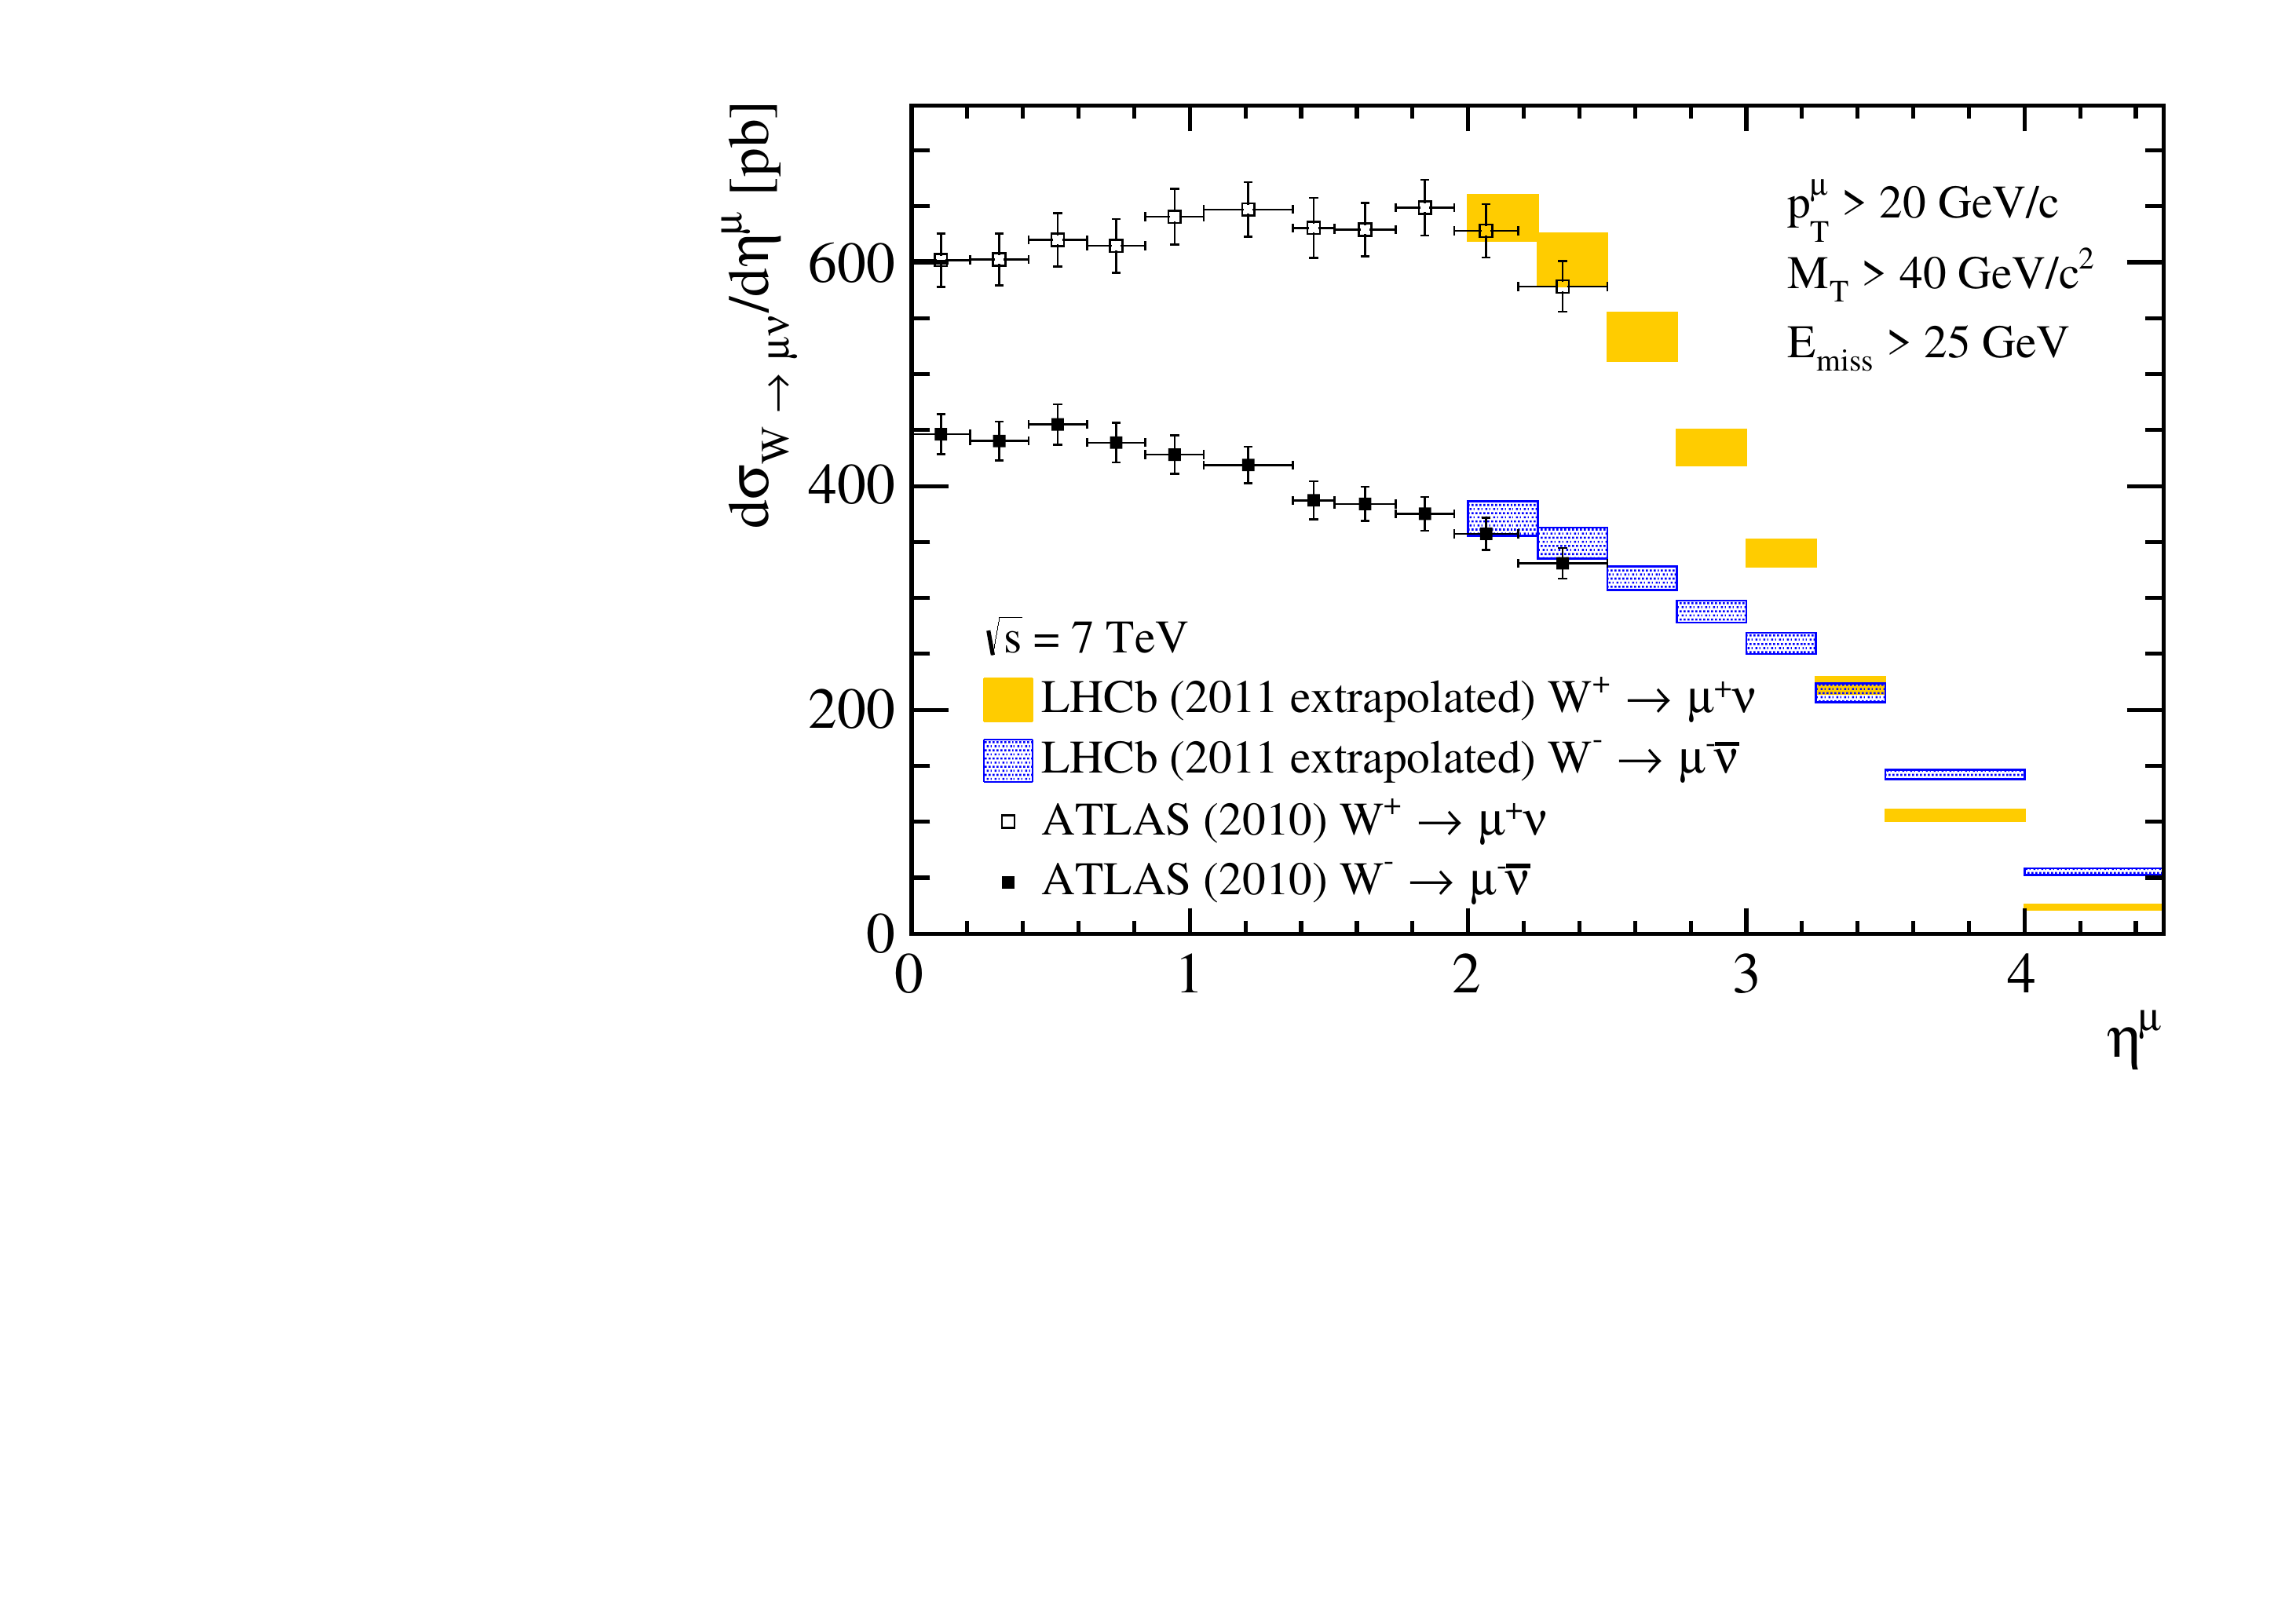}
  \end{center}
  \caption{
   Extrapolation of \lhcb \PW boson cross-section measurements to the ATLAS fiducial volume (muons with $\pt > 20$ \gevc
and invariant mass $66<M_{\mu\mu}<116$ \gevcc)~\cite{atlaswz}.
  }
  \label{fig:cswc}
\end{figure}

\clearpage

\begin{figure}[!t]
\begin{center}
\includegraphics[width=\textwidth]{./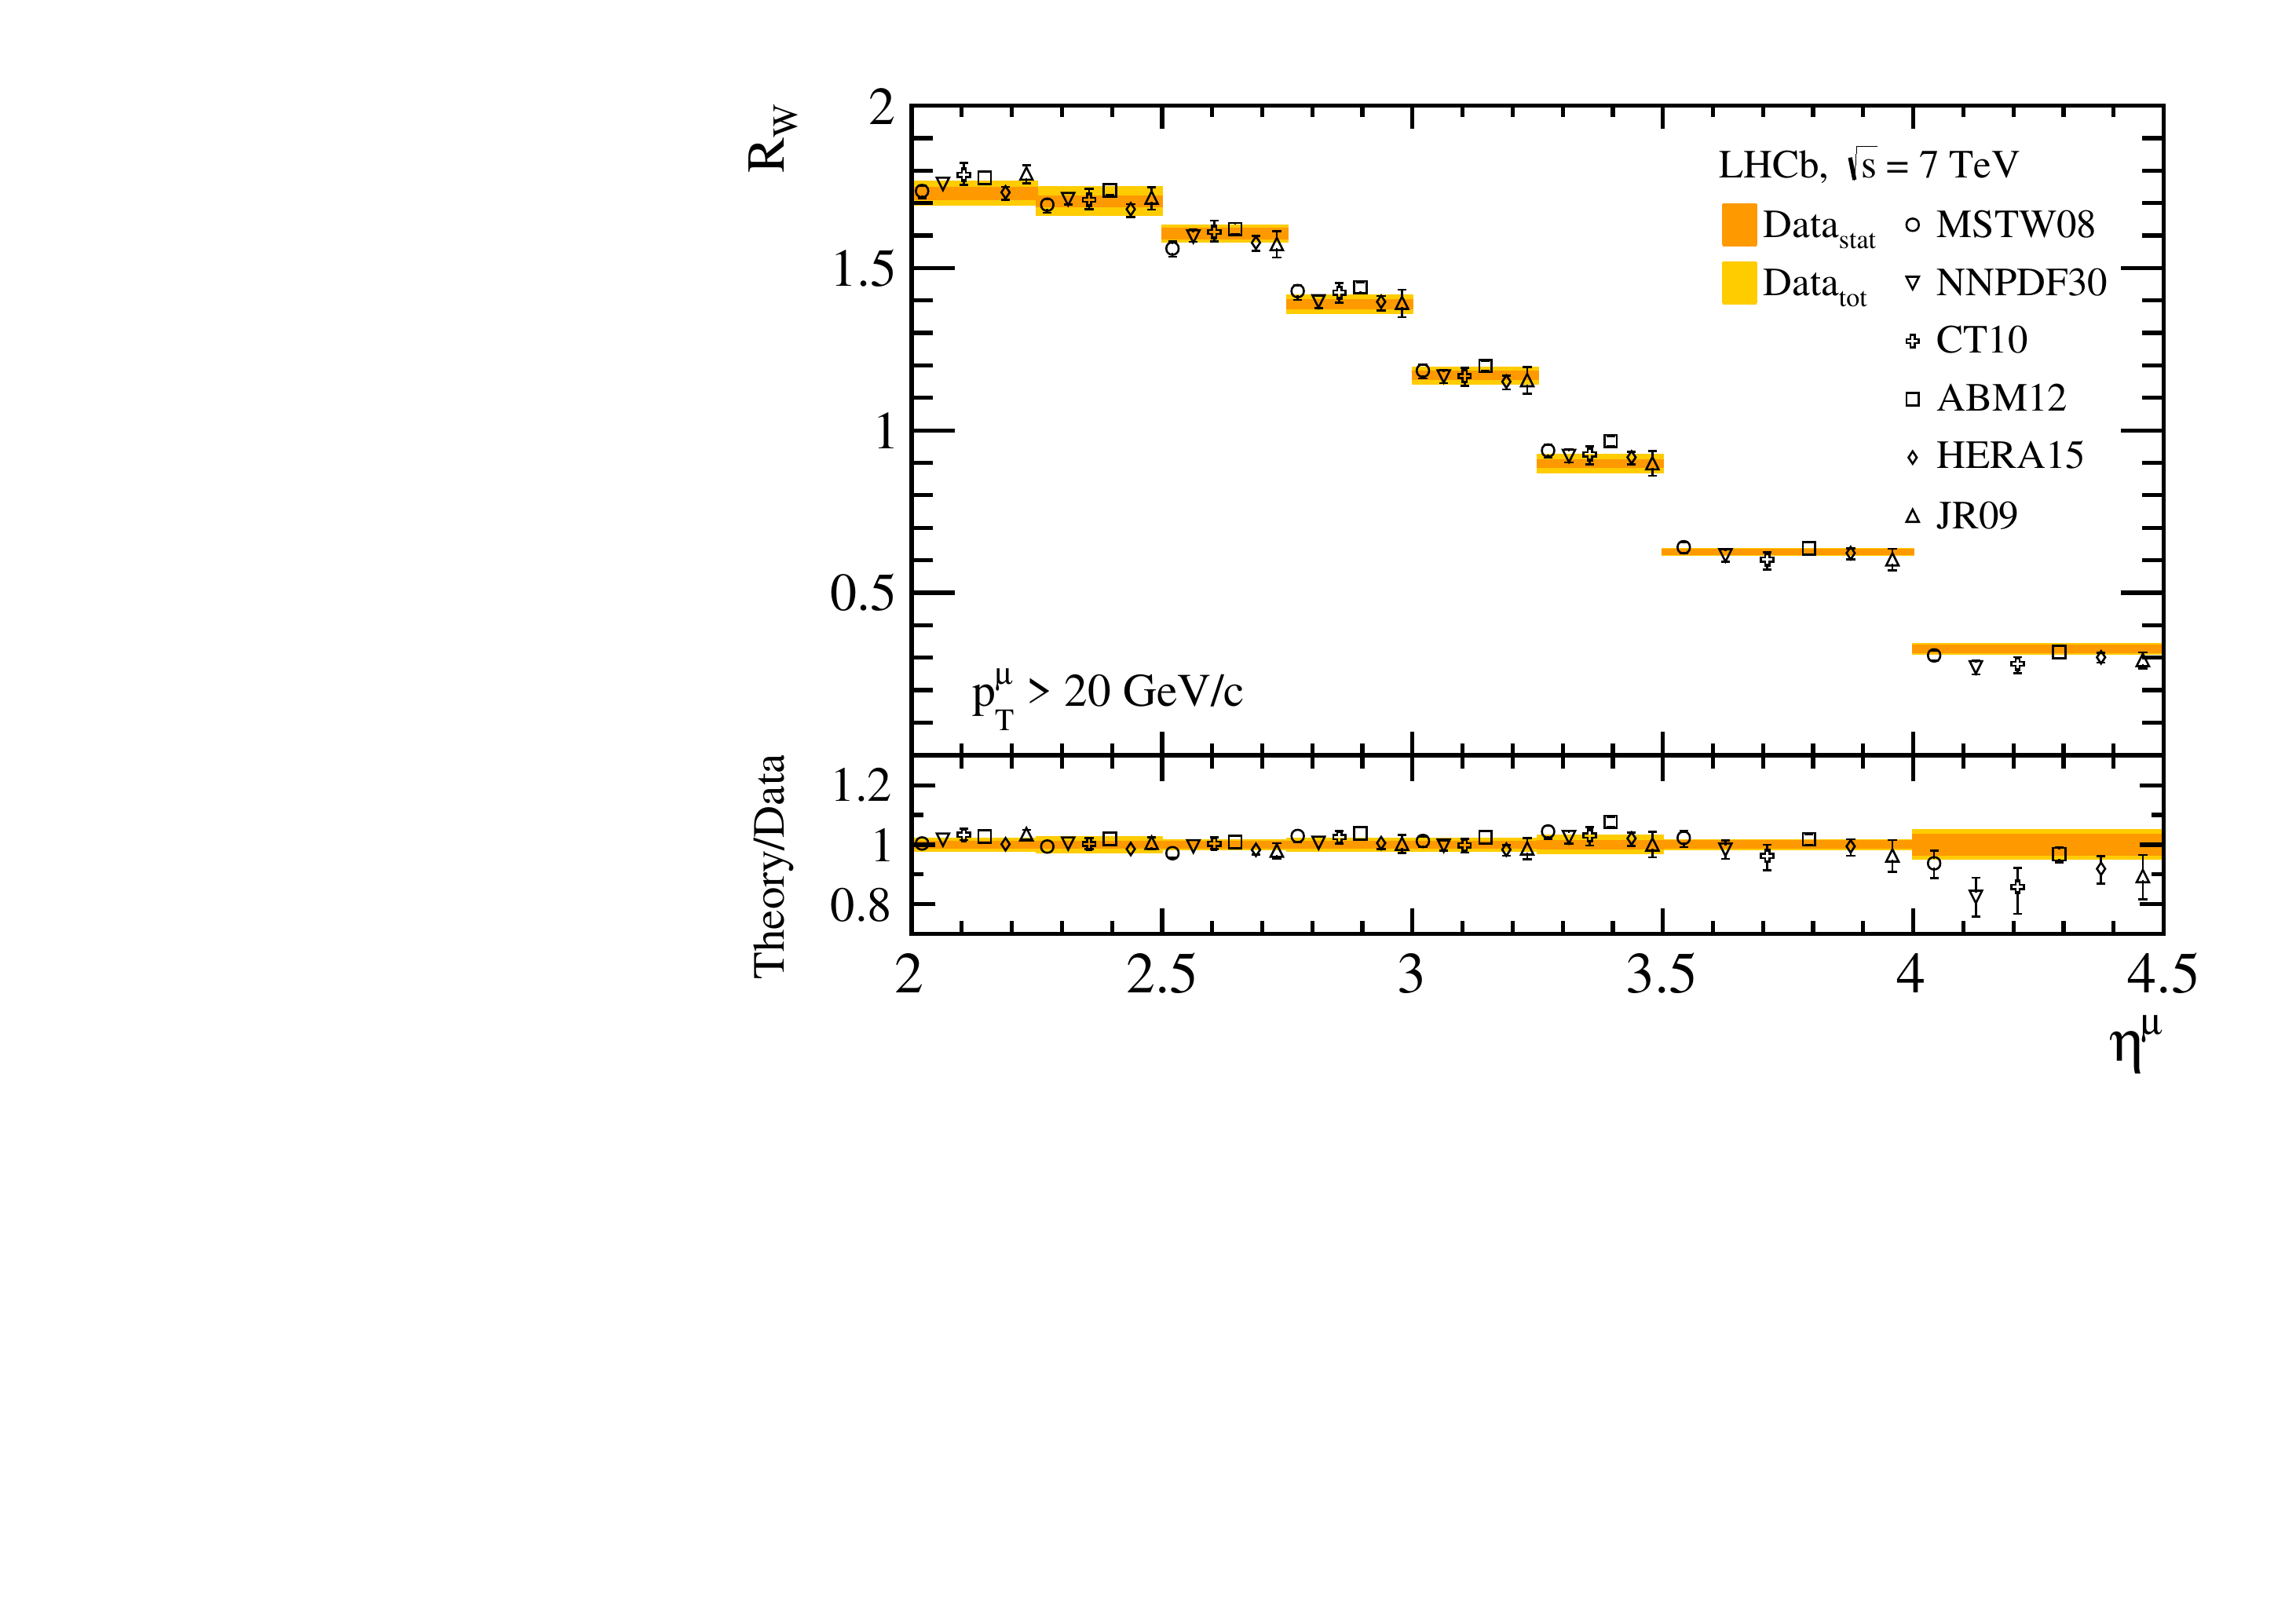}
\caption{\Wp to \Wm cross-section ratios as a function of muon $\eta$. 
Measurements, represented as bands corresponding 
to 
the (orange) statistical and (yellow) total uncertainty, are compared to (black markers, displaced horizontally for presentation) NNLO predictions with different parameterisations of the PDFs.}
\end{center}
\end{figure}

\clearpage
\begin{figure}[!t]
\begin{center}
\includegraphics[width=\textwidth]{./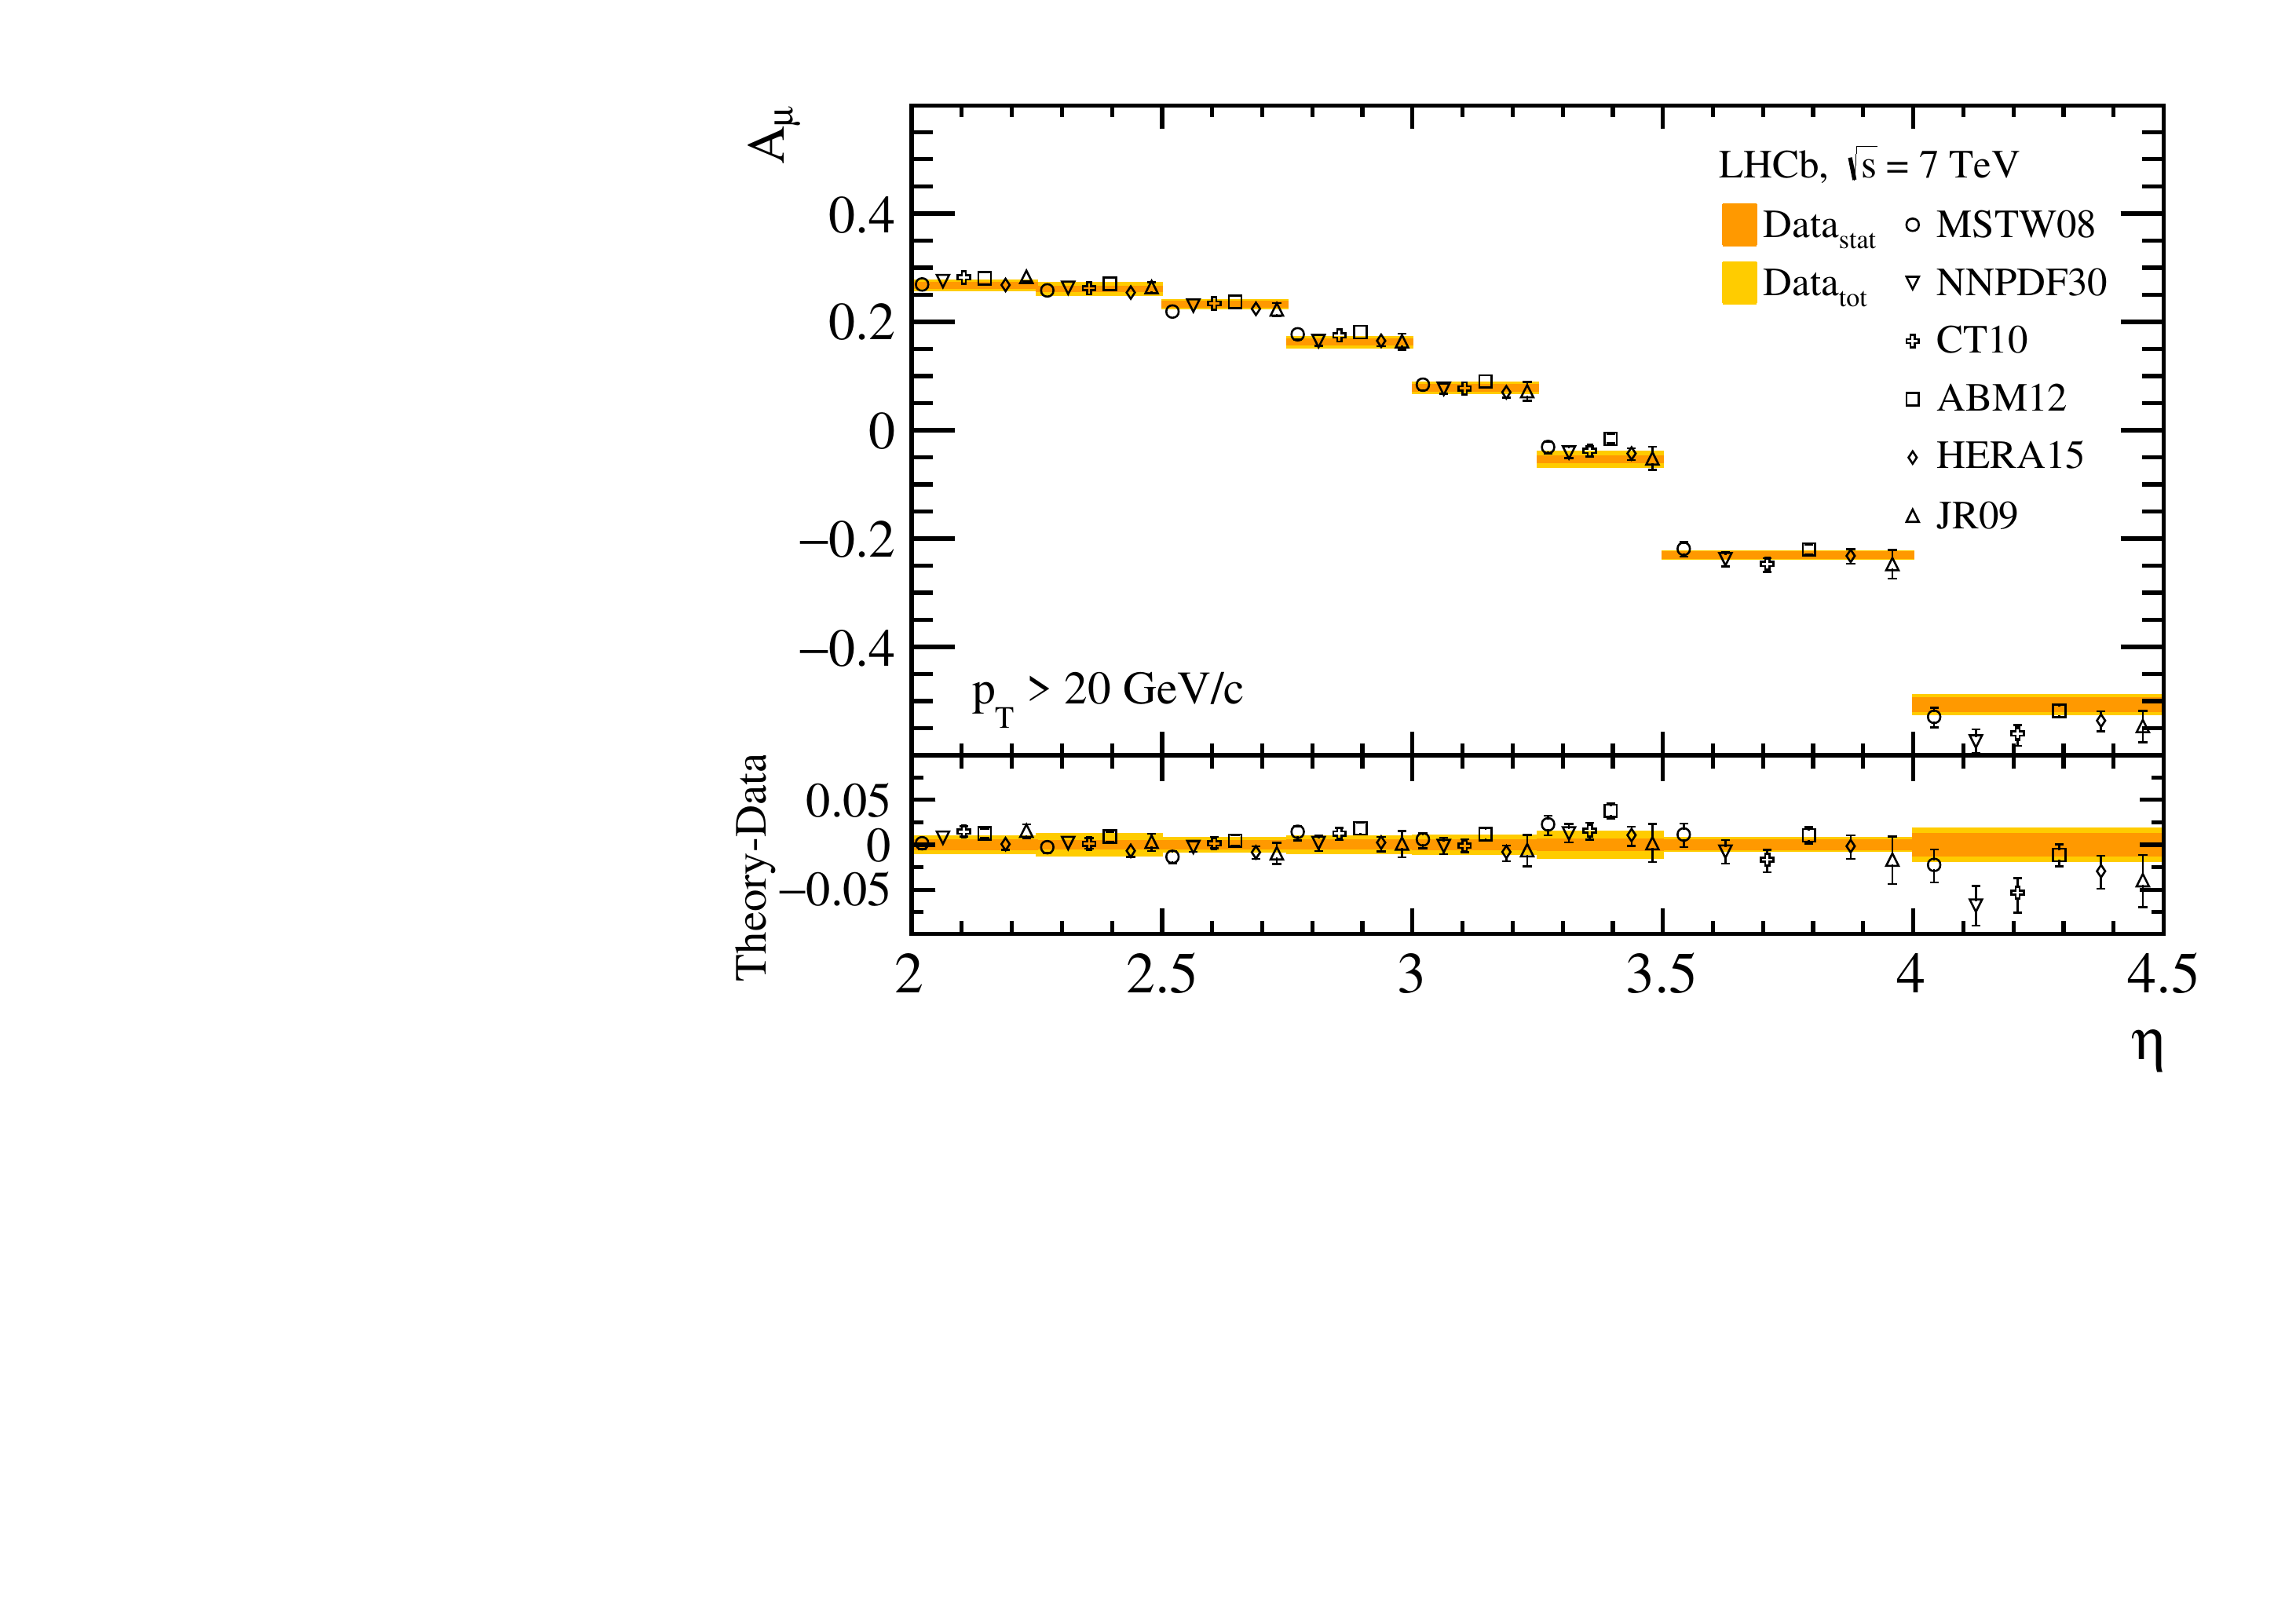}
\caption{Lepton charge asymmetries in \PW decays as a function of muon $\eta$. 
Measurements, represented as bands corresponding to 
the 
(orange) statistical and (yellow) total uncertainty, are compared to (open 
black markers, displaced horizontally for presentation) NNLO predictions with different parameterisations of the PDFs.}
\end{center}
\end{figure}

\clearpage
\begin{figure}[!t]
\begin{center}
\includegraphics[width=\textwidth]{./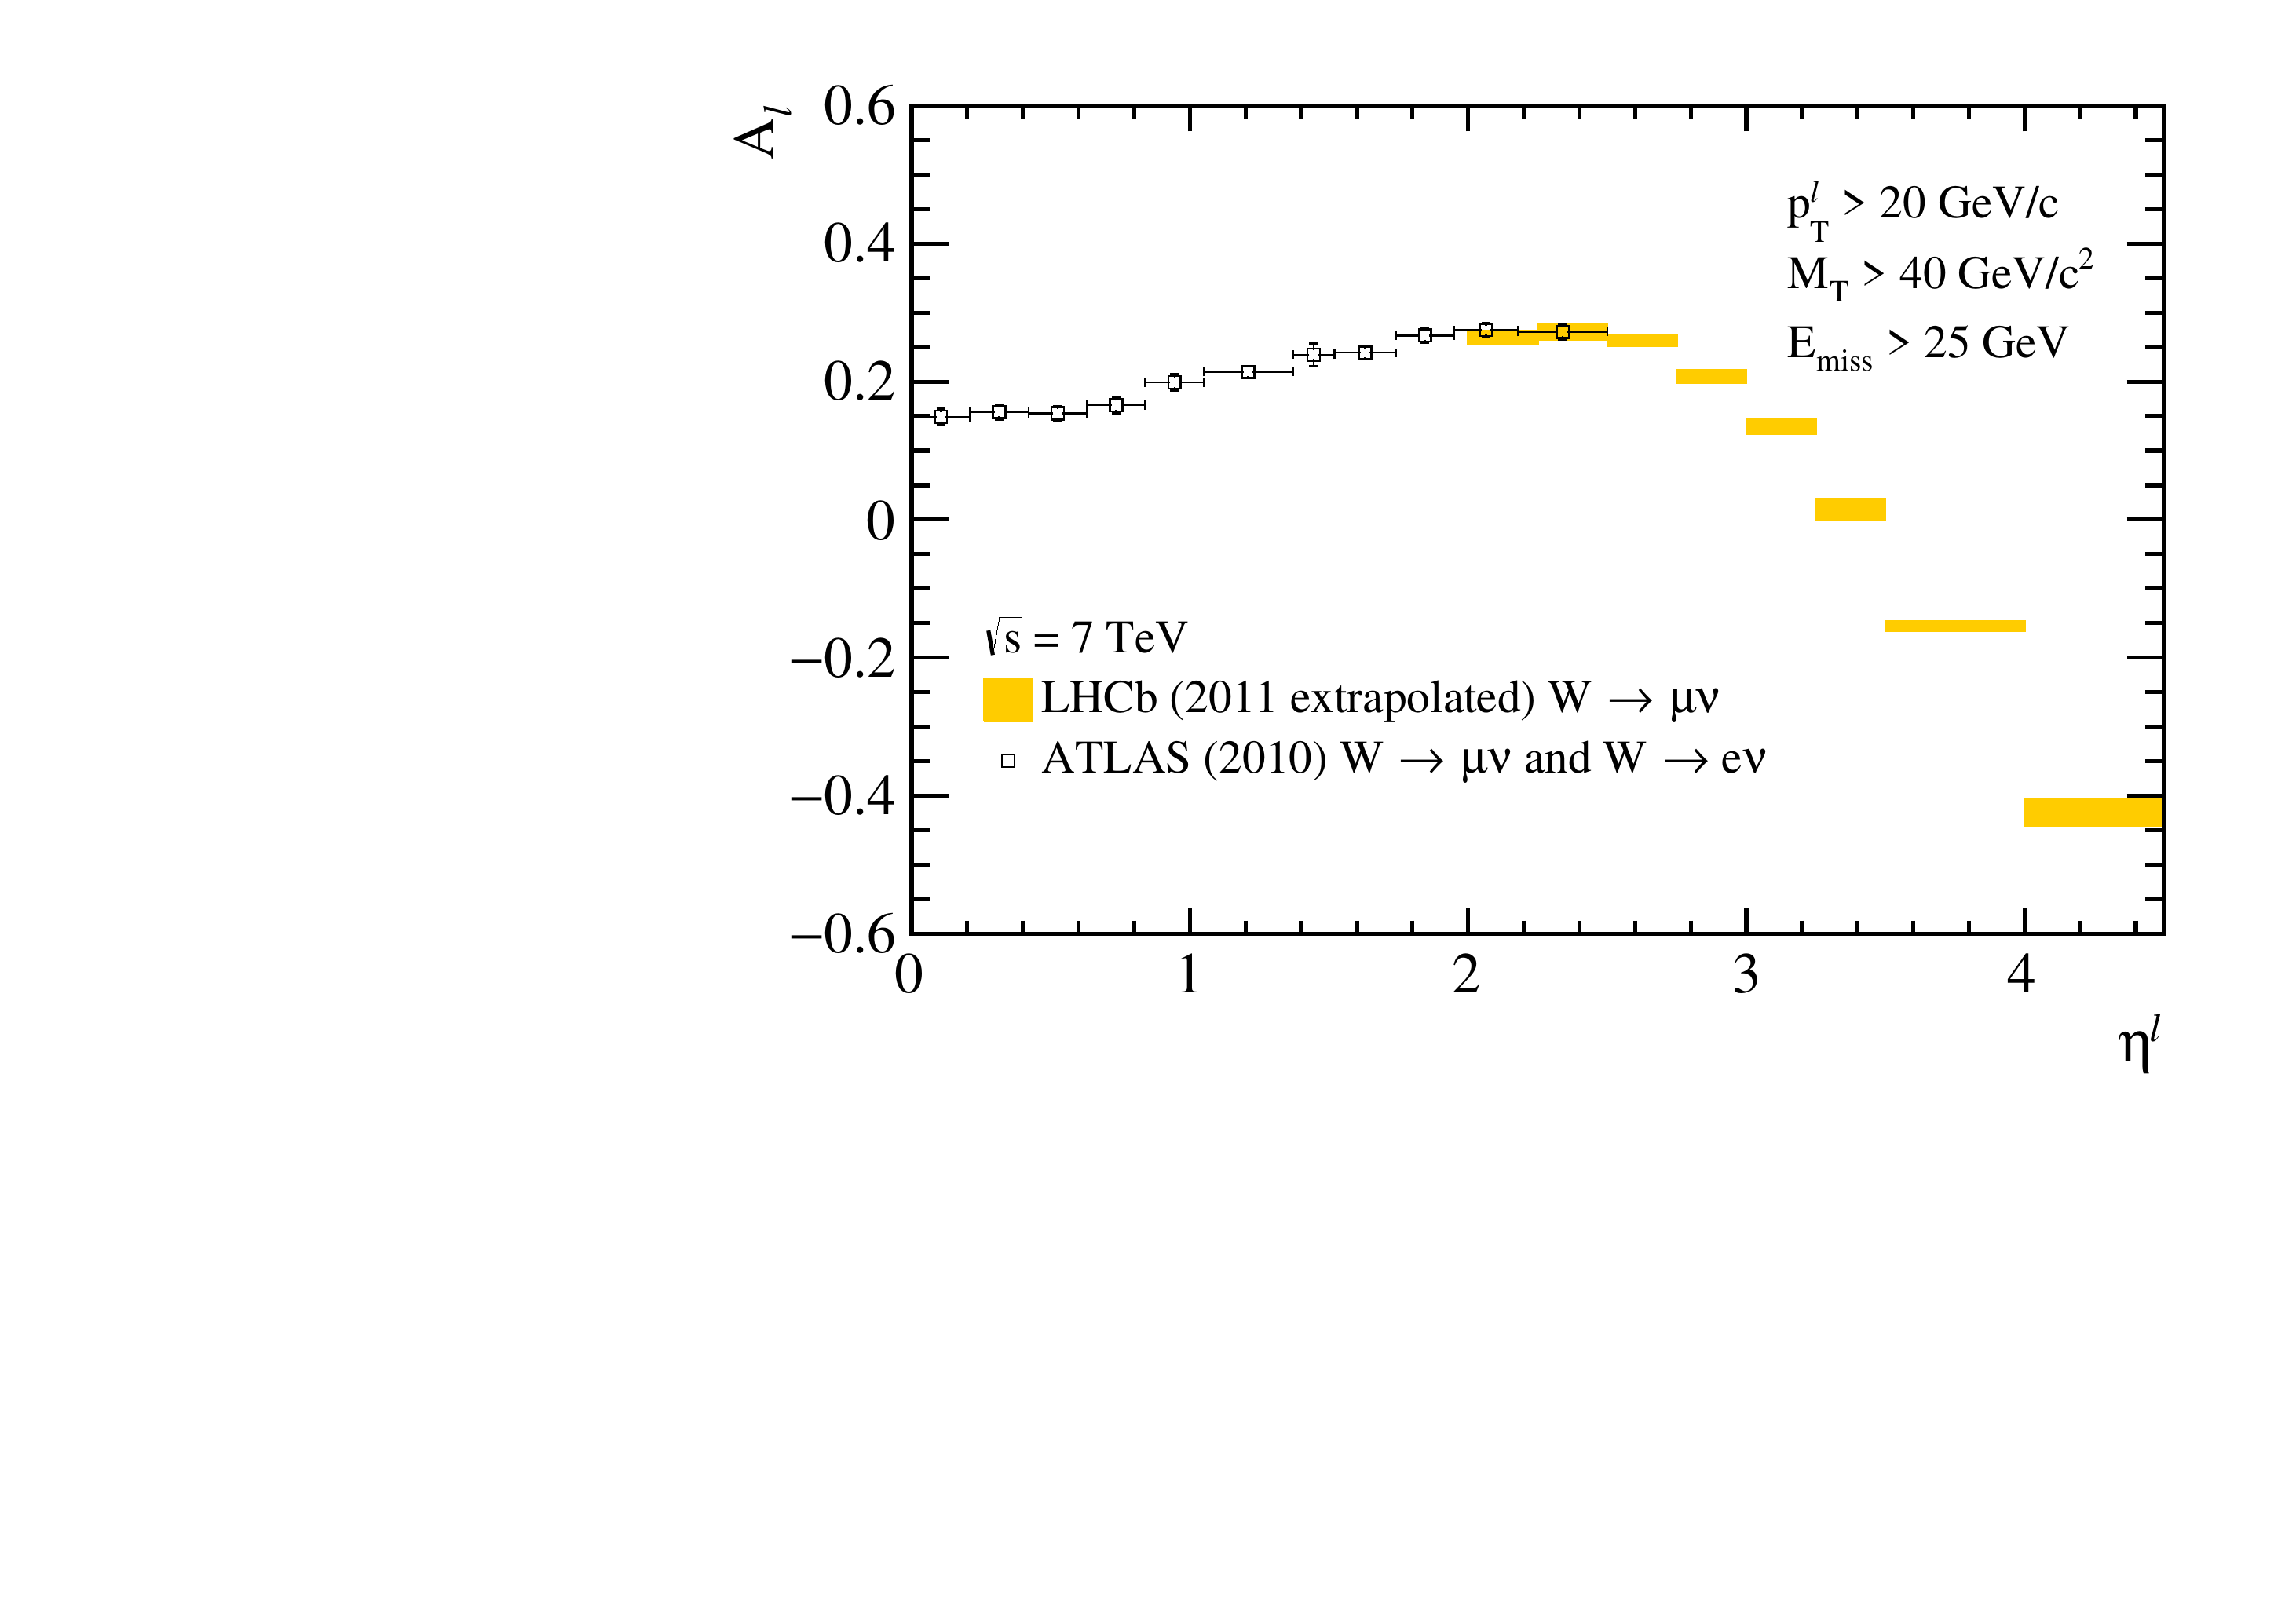}
\caption{Lepton charge asymmetries in \PW decays as a function of muon $\eta$. 
Measurements, represented as bands corresponding to 
the (yellow) total uncertainty, are extrapolated to the ATLAS fiducial 
volume ($M_{\textrm{T}} > 40\gevcc$ and $E_{\textrm{miss}} > 25\gev$) and 
compared to the (open black markers) ATLAS determinations~\cite{atlaswz}.}
\end{center}
\end{figure}

\clearpage
\begin{figure}[!t]
\begin{center}
\includegraphics[width=\textwidth]{./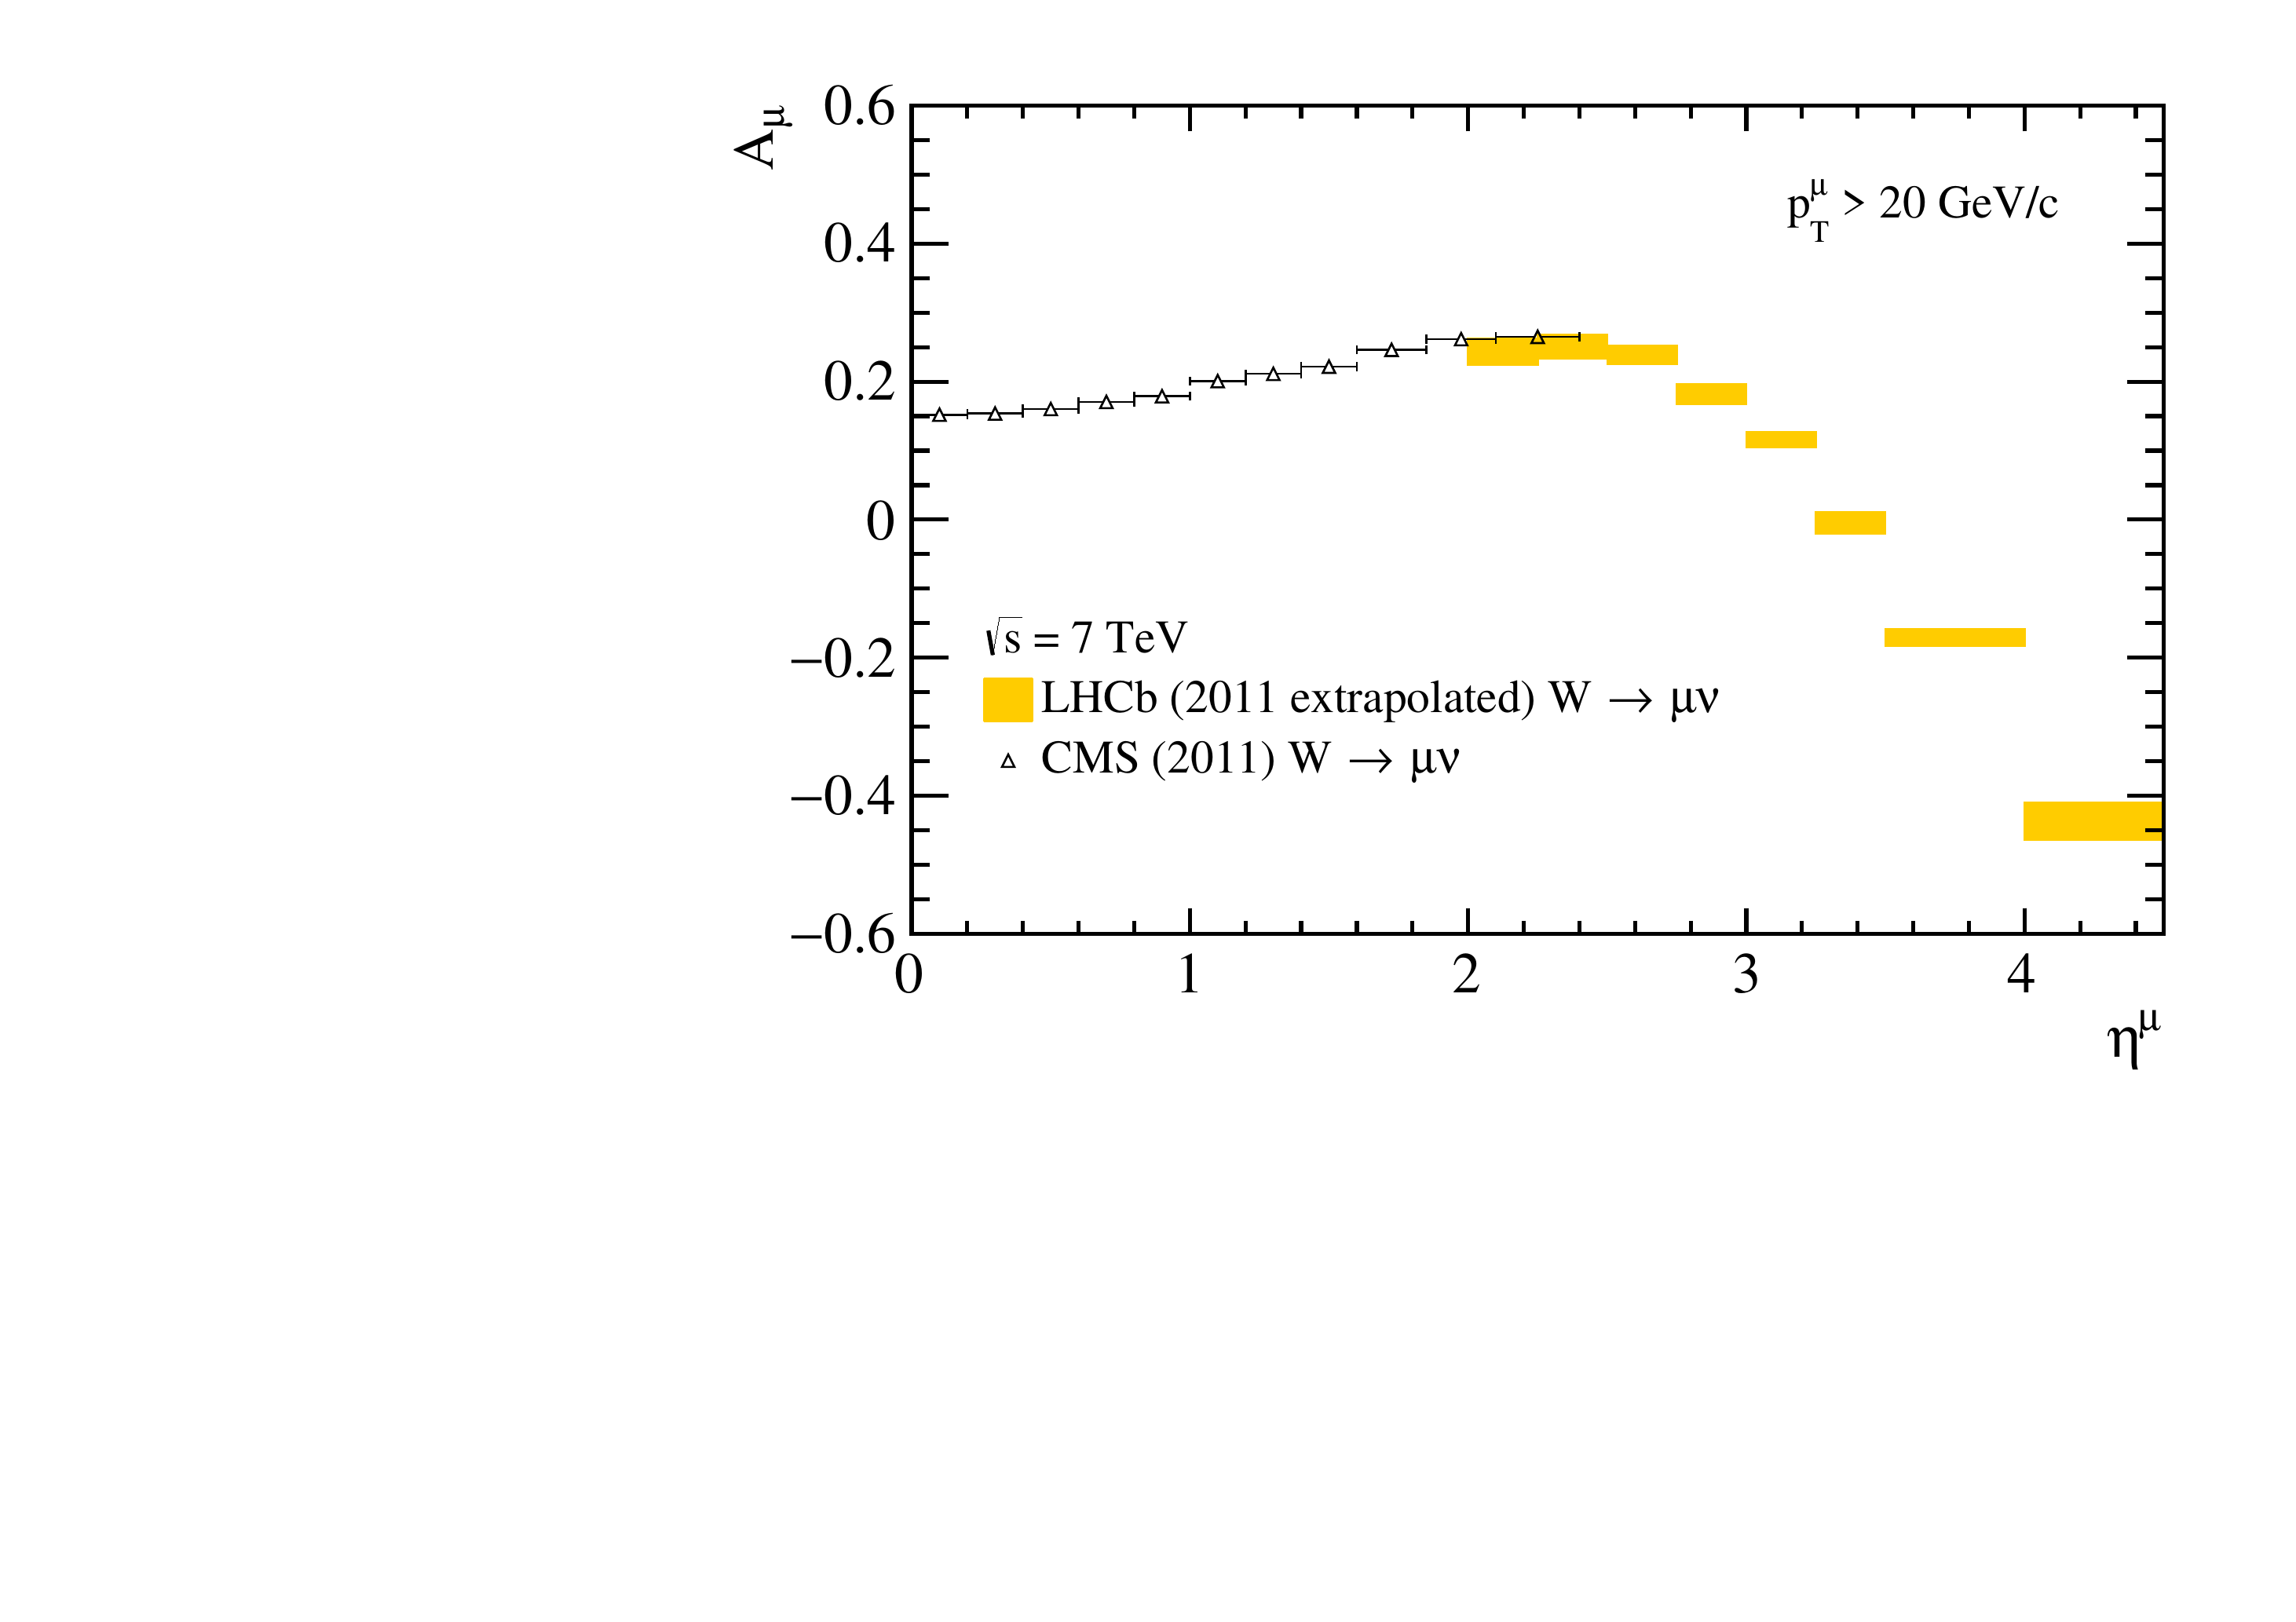}
\caption{Lepton charge asymmetries in \PW decays as a function of muon $\eta$. 
Measurements, represented as bands corresponding to 
the (yellow) total uncertainty, are extrapolated to the CMS fiducial volume 
($\pt > 25\gevc$) and compared to the (open black markers) CMS 
determinations~\cite{CMSAsymm}.} \end{center}
\end{figure}

\clearpage
