# Supplementary material for: Measurement of the forward $Z$ boson production cross-section in $pp$ collisions at $\sqrt{s}$ = 7 TeV
Source: arXiv:1505.07024 source file (2015-08-20)
Supplement: Supplementary file 2 [file supplementary.tex]

\section{Inclusion of supplementary material}
\label{sec:Supplementary}

Three types of supplementary material should be distinguised:
\begin{itemize}
\item{A regular appendix: lengthy equations or long tables are sometimes
better put in an appendix in order not to interrupt the main flow of a paper.
Appendices will appear in the final paper, on arXiv
and on the cds record and should be considered integral
part of a paper, and are thus to be reviewed like the rest of the paper.
An example of an LHCb paper with an appendix is Ref.~\cite{LHCb-PAPER-2013-070}.
}
\item{Supplementary material for cds: plots or tables that 
would make the paper exceed the page limit or are
not appropriate to include in the paper itself,
but are desireable to be shown in public
should be added to the paper drafts in an appendix, and
removed from the paper before submitting to arXiv or the journal.
See Appendix~\ref{sec:Supplementary-App} for further instructions.
Examples are: comparison plots of the new result with older results,
plots that illustrate cross-checks.
An example of an LHCb paper with supplementary material for cds 
is Ref.~\cite{LHCb-PAPER-2013-035}.
Supplementary material for cds cannot be referenced to in the paper.
}
\item{Supplementary material for the paper. Most journals allow
to submit files along with the paper that will not be part of the
text of the article, but will be stored on the journal server.
Examples are plain text files with numerical data corresponding to the plots
in the paper. 
The supplementary material should be referenced to in the paper, by including a reference
of the type  ``See supplementary material for [give brief description of material].''
The journal will insert a specific link here. For the arXiv record, 
a specific link to the supplementary material on the arXiv server should be 
included when the paper gets updated, after it has been published.
For the internal reviewing, an appendix should be provided illustrating
the format of the file, its purpose and providing a link where the actual
files can be found.
An example of an LHCb paper with supplementary material is Ref.~\cite{LHCb-PAPER-2011-020}
}
\end{itemize}
